# Supplementary material for: An Evolutionary Algorithm Assisted by an Ensemble of Pareto-Optimal Surrogate Models
Source: arXiv:2608.01777 source file (2026-08-03)
Supplement: Supplementary file 1 [file main.tex]

%% bare_jrnl.tex
%% V1.4b
%% 2015/08/26
%% by Michael Shell
%% see http://www.michaelshell.org/
%% for current contact information.
%%
%% This is a skeleton file demonstrating the use of IEEEtran.cls
%% (requires IEEEtran.cls version 1.8b or later) with an IEEE
%% journal paper.
%%
%% Support sites:
%% http://www.michaelshell.org/tex/ieeetran/
%% http://www.ctan.org/pkg/ieeetran
%% and
%% http://www.ieee.org/

%%*************************************************************************
%% Legal Notice:
%% This code is offered as-is without any warranty either expressed or
%% implied; without even the implied warranty of MERCHANTABILITY or
%% FITNESS FOR A PARTICULAR PURPOSE! 
%% User assumes all risk.
%% In no event shall the IEEE or any contributor to this code be liable for
%% any damages or losses, including, but not limited to, incidental,
%% consequential, or any other damages, resulting from the use or misuse
%% of any information contained here.
%%
%% All comments are the opinions of their respective authors and are not
%% necessarily endorsed by the IEEE.
%%
%% This work is distributed under the LaTeX Project Public License (LPPL)
%% ( http://www.latex-project.org/ ) version 1.3, and may be freely used,
%% distributed and modified. A copy of the LPPL, version 1.3, is included
%% in the base LaTeX documentation of all distributions of LaTeX released
%% 2003/12/01 or later.
%% Retain all contribution notices and credits.
%% ** Modified files should be clearly indicated as such, including  **
%% ** renaming them and changing author support contact information. **
%%*************************************************************************


% *** Authors should verify (and, if needed, correct) their LaTeX system  ***
% *** with the testflow diagnostic prior to trusting their LaTeX platform ***
% *** with production work. The IEEE's font choices and paper sizes can   ***
% *** trigger bugs that do not appear when using other class files.       ***                          ***
% The testflow support page is at:
% http://www.michaelshell.org/tex/testflow/



\documentclass[journal,twoside]{IEEEtran}
%
% If IEEEtran.cls has not been installed into the LaTeX system files,
% manually specify the path to it like:
% \documentclass[journal]{../sty/IEEEtran}





% Some very useful LaTeX packages include:
% (uncomment the ones you want to load)


% *** MISC UTILITY PACKAGES ***
%
%\usepackage{ifpdf}
% Heiko Oberdiek's ifpdf.sty is very useful if you need conditional
% compilation based on whether the output is pdf or dvi.
% usage:
% \ifpdf
%   % pdf code
% \else
%   % dvi code
% \fi
% The latest version of ifpdf.sty can be obtained from:
% http://www.ctan.org/pkg/ifpdf
% Also, note that IEEEtran.cls V1.7 and later provides a builtin
% \ifCLASSINFOpdf conditional that works the same way.
% When switching from latex to pdflatex and vice-versa, the compiler may
% have to be run twice to clear warning/error messages.






% *** CITATION PACKAGES ***
%
\usepackage{cite}
% cite.sty was written by Donald Arseneau
% V1.6 and later of IEEEtran pre-defines the format of the cite.sty package
% \cite{} output to follow that of the IEEE. Loading the cite package will
% result in citation numbers being automatically sorted and properly
% "compressed/ranged". e.g., [1], [9], [2], [7], [5], [6] without using
% cite.sty will become [1], [2], [5]--[7], [9] using cite.sty. cite.sty's
% \cite will automatically add leading space, if needed. Use cite.sty's
% noadjust option (cite.sty V3.8 and later) if you want to turn this off
% such as if a citation ever needs to be enclosed in parenthesis.
% cite.sty is already installed on most LaTeX systems. Be sure and use
% version 5.0 (2009-03-20) and later if using hyperref.sty.
% The latest version can be obtained at:
% http://www.ctan.org/pkg/cite
% The documentation is contained in the cite.sty file itself.






% *** GRAPHICS RELATED PACKAGES ***
%
\ifCLASSINFOpdf
   \usepackage[pdftex]{graphicx}
  % declare the path(s) where your graphic files are
  % \graphicspath{{../pdf/}{../jpeg/}}
  % and their extensions so you won't have to specify these with
  % every instance of \includegraphics
  % \DeclareGraphicsExtensions{.pdf,.jpeg,.png}
\else
  % or other class option (dvipsone, dvipdf, if not using dvips). graphicx
  % will default to the driver specified in the system graphics.cfg if no
  % driver is specified.
  % \usepackage[dvips]{graphicx}
  % declare the path(s) where your graphic files are
  % \graphicspath{{../eps/}}
  % and their extensions so you won't have to specify these with
  % every instance of \includegraphics
  % \DeclareGraphicsExtensions{.eps}
\fi
% graphicx was written by David Carlisle and Sebastian Rahtz. It is
% required if you want graphics, photos, etc. graphicx.sty is already
% installed on most LaTeX systems. The latest version and documentation
% can be obtained at: 
% http://www.ctan.org/pkg/graphicx
% Another good source of documentation is "Using Imported Graphics in
% LaTeX2e" by Keith Reckdahl which can be found at:
% http://www.ctan.org/pkg/epslatex
%
% latex, and pdflatex in dvi mode, support graphics in encapsulated
% postscript (.eps) format. pdflatex in pdf mode supports graphics
% in .pdf, .jpeg, .png and .mps (metapost) formats. Users should ensure
% that all non-photo figures use a vector format (.eps, .pdf, .mps) and
% not a bitmapped formats (.jpeg, .png). The IEEE frowns on bitmapped formats
% which can result in "jaggedy"/blurry rendering of lines and letters as
% well as large increases in file sizes.
%
% You can find documentation about the pdfTeX application at:
% http://www.tug.org/applications/pdftex


% *** MATH PACKAGES ***
%
\usepackage{amsmath,amssymb}
\DeclareMathOperator*{\argmax}{arg\hspace{1pt}max} 
\DeclareMathOperator*{\argmin}{arg\hspace{1pt}min} 
% A popular package from the American Mathematical Society that provides
% many useful and powerful commands for dealing with mathematics.
%
% Note that the amsmath package sets \interdisplaylinepenalty to 10000
% thus preventing page breaks from occurring within multiline equations. Use:
%\interdisplaylinepenalty=2500
% after loading amsmath to restore such page breaks as IEEEtran.cls normally
% does. amsmath.sty is already installed on most LaTeX systems. The latest
% version and documentation can be obtained at:
% http://www.ctan.org/pkg/amsmath





% *** SPECIALIZED LIST PACKAGES ***
%
%\usepackage{algorithmic}
% algorithmic.sty was written by Peter Williams and Rogerio Brito.
% This package provides an algorithmic environment fo describing algorithms.
% You can use the algorithmic environment in-text or within a figure
% environment to provide for a floating algorithm. Do NOT use the algorithm
% floating environment provided by algorithm.sty (by the same authors) or
% algorithm2e.sty (by Christophe Fiorio) as the IEEE does not use dedicated
% algorithm float types and packages that provide these will not provide
% correct IEEE style captions. The latest version and documentation of
% algorithmic.sty can be obtained at:
% http://www.ctan.org/pkg/algorithms
% Also of interest may be the (relatively newer and more customizable)
% algorithmicx.sty package by Szasz Janos:
% http://www.ctan.org/pkg/algorithmicx




% *** ALIGNMENT PACKAGES ***
%
%\usepackage{array}
% Frank Mittelbach's and David Carlisle's array.sty patches and improves
% the standard LaTeX2e array and tabular environments to provide better
% appearance and additional user controls. As the default LaTeX2e table
% generation code is lacking to the point of almost being broken with
% respect to the quality of the end results, all users are strongly
% advised to use an enhanced (at the very least that provided by array.sty)
% set of table tools. array.sty is already installed on most systems. The
% latest version and documentation can be obtained at:
% http://www.ctan.org/pkg/array


% IEEEtran contains the IEEEeqnarray family of commands that can be used to
% generate multiline equations as well as matrices, tables, etc., of high
% quality.




% *** SUBFIGURE PACKAGES ***
%\ifCLASSOPTIONcompsoc
%  \usepackage[caption=false,font=normalsize,labelfont=sf,textfont=sf]{subfig}
%\else
%  \usepackage[caption=false,font=footnotesize]{subfig}
%\fi
% subfig.sty, written by Steven Douglas Cochran, is the modern replacement
% for subfigure.sty, the latter of which is no longer maintained and is
% incompatible with some LaTeX packages including fixltx2e. However,
% subfig.sty requires and automatically loads Axel Sommerfeldt's caption.sty
% which will override IEEEtran.cls' handling of captions and this will result
% in non-IEEE style figure/table captions. To prevent this problem, be sure
% and invoke subfig.sty's "caption=false" package option (available since
% subfig.sty version 1.3, 2005/06/28) as this is will preserve IEEEtran.cls
% handling of captions.
% Note that the Computer Society format requires a larger sans serif font
% than the serif footnote size font used in traditional IEEE formatting
% and thus the need to invoke different subfig.sty package options depending
% on whether compsoc mode has been enabled.
%
% The latest version and documentation of subfig.sty can be obtained at:
% http://www.ctan.org/pkg/subfig




% *** FLOAT PACKAGES ***
%
%\usepackage{fixltx2e}
% fixltx2e, the successor to the earlier fix2col.sty, was written by
% Frank Mittelbach and David Carlisle. This package corrects a few problems
% in the LaTeX2e kernel, the most notable of which is that in current
% LaTeX2e releases, the ordering of single and double column floats is not
% guaranteed to be preserved. Thus, an unpatched LaTeX2e can allow a
% single column figure to be placed prior to an earlier double column
% figure.
% Be aware that LaTeX2e kernels dated 2015 and later have fixltx2e.sty's
% corrections already built into the system in which case a warning will
% be issued if an attempt is made to load fixltx2e.sty as it is no longer
% needed.
% The latest version and documentation can be found at:
% http://www.ctan.org/pkg/fixltx2e


%\usepackage{stfloats}
% stfloats.sty was written by Sigitas Tolusis. This package gives LaTeX2e
% the ability to do double column floats at the bottom of the page as well
% as the top. (e.g., "\begin{figure*}[!b]" is not normally possible in
% LaTeX2e). It also provides a command:
%\fnbelowfloat
% to enable the placement of footnotes below bottom floats (the standard
% LaTeX2e kernel puts them above bottom floats). This is an invasive package
% which rewrites many portions of the LaTeX2e float routines. It may not work
% with other packages that modify the LaTeX2e float routines. The latest
% version and documentation can be obtained at:
% http://www.ctan.org/pkg/stfloats
% Do not use the stfloats baselinefloat ability as the IEEE does not allow
% \baselineskip to stretch. Authors submitting work to the IEEE should note
% that the IEEE rarely uses double column equations and that authors should try
% to avoid such use. Do not be tempted to use the cuted.sty or midfloat.sty
% packages (also by Sigitas Tolusis) as the IEEE does not format its papers in
% such ways.
% Do not attempt to use stfloats with fixltx2e as they are incompatible.
% Instead, use Morten Hogholm'a dblfloatfix which combines the features
% of both fixltx2e and stfloats:
%
% \usepackage{dblfloatfix}
% The latest version can be found at:
% http://www.ctan.org/pkg/dblfloatfix




%\ifCLASSOPTIONcaptionsoff
%  \usepackage[nomarkers]{endfloat}
% \let\MYoriglatexcaption\caption
% \renewcommand{\caption}[2][\relax]{\MYoriglatexcaption[#2]{#2}}
%\fi
% endfloat.sty was written by James Darrell McCauley, Jeff Goldberg and 
% Axel Sommerfeldt. This package may be useful when used in conjunction with 
% IEEEtran.cls'  captionsoff option. Some IEEE journals/societies require that
% submissions have lists of figures/tables at the end of the paper and that
% figures/tables without any captions are placed on a page by themselves at
% the end of the document. If needed, the draftcls IEEEtran class option or
% \CLASSINPUTbaselinestretch interface can be used to increase the line
% spacing as well. Be sure and use the nomarkers option of endfloat to
% prevent endfloat from "marking" where the figures would have been placed
% in the text. The two hack lines of code above are a slight modification of
% that suggested by in the endfloat docs (section 8.4.1) to ensure that
% the full captions always appear in the list of figures/tables - even if
% the user used the short optional argument of \caption[]{}.
% IEEE papers do not typically make use of \caption[]'s optional argument,
% so this should not be an issue. A similar trick can be used to disable
% captions of packages such as subfig.sty that lack options to turn off
% the subcaptions:
% For subfig.sty:
% \let\MYorigsubfloat\subfloat
% \renewcommand{\subfloat}[2][\relax]{\MYorigsubfloat[]{#2}}
% However, the above trick will not work if both optional arguments of
% the \subfloat command are used. Furthermore, there needs to be a
% description of each subfigure *somewhere* and endfloat does not add
% subfigure captions to its list of figures. Thus, the best approach is to
% avoid the use of subfigure captions (many IEEE journals avoid them anyway)
% and instead reference/explain all the subfigures within the main caption.
% The latest version of endfloat.sty and its documentation can obtained at:
% http://www.ctan.org/pkg/endfloat
%
% The IEEEtran \ifCLASSOPTIONcaptionsoff conditional can also be used
% later in the document, say, to conditionally put the References on a 
% page by themselves.




% *** PDF, URL AND HYPERLINK PACKAGES ***
%
\usepackage{url}
% url.sty was written by Donald Arseneau. It provides better support for
% handling and breaking URLs. url.sty is already installed on most LaTeX
% systems. The latest version and documentation can be obtained at:
% http://www.ctan.org/pkg/url
% Basically, \url{my_url_here}.




% *** Do not adjust lengths that control margins, column widths, etc. ***
% *** Do not use packages that alter fonts (such as pslatex).         ***
% There should be no need to do such things with IEEEtran.cls V1.6 and later.
% (Unless specifically asked to do so by the journal or conference you plan
% to submit to, of course. )


% correct bad hyphenation here
\hyphenation{}


%%% added package BEGIN %%%

\usepackage{longtable}
\usepackage[noend]{algorithmic}
\usepackage{algorithm}
\usepackage{subfigure}
\usepackage{array}
\usepackage{textcomp}
\usepackage{stfloats}
\usepackage{verbatim}
\usepackage{cite}
\usepackage{color, xcolor, colortbl}
\usepackage{bm}
\usepackage{multirow}
\usepackage{multicol}
\usepackage{latexsym}
\usepackage{arydshln}
\usepackage{afterpage}
\usepackage{booktabs}
\usepackage[hidelinks]{hyperref}
% \hypersetup{
%     setpagesize=false,
%     bookmarksnumbered=true,%
%     bookmarksopen=true,%
%     colorlinks=true,%
%     linkcolor=black,
%     citecolor=black,
% }
\usepackage{ulem}

\usepackage{xr}
\externaldocument{../main}
\renewcommand{\thesection}{S-\Roman{section}}
\renewcommand{\theequation}{S-\arabic{equation}}
\renewcommand{\thetable}{S-\Roman{table}}
\renewcommand{\thefigure}{S-\arabic{figure}}
\renewcommand{\thealgorithm}{S-\arabic{algorithm}}

\definecolor{mygreen}{rgb}{0.93,0.96,0.82} % 0.81,0.88,0.51
\definecolor{mypink}{rgb}{0.98,0.91,0.92}
\definecolor{myyellow}{rgb}{0.99,0.95,0.72}

% \newcommand{\w}{\cellcolor{mygreen}\bfseries} 
\newcommand{\w}{\cellcolor{mygreen}} 
\newcommand{\ls}{\cellcolor{mypink}}
% \newcommand{\ls}{}
\newcommand{\m}{\cellcolor{myyellow}}

\newcommand{\win}{\cellcolor{mygreen}\bfseries} 
\newcommand{\worst}{\cellcolor{mypink}\it}
% \newcommand{\worst}{}

\newcommand{\mygreen}[1]{\colorbox{mygreen}{#1}}
\newcommand{\mypink}[1]{\colorbox{mypink}{#1}}
% \newcommand{\red}[1]{\textcolor{red}{#1}}
\newcommand{\red}[1]{\textcolor{black}{#1}}
\newcommand{\blue}[1]{\textcolor{blue}{#1}}
\definecolor{green2}{rgb}{ .23, .68, .46}
\newcommand{\green}[1]{\textcolor{green2}{#1}}

\newcommand{\plus}{$+$}
\newcommand{\minus}{$-$}
\newcommand{\nodiff}{$\sim$}

\newcommand{\cth}{\multicolumn{1}{c}}
\newcommand{\cttd}{\multicolumn{2}{c:}}
\newcommand{\cttl}{\multicolumn{2}{c|}}

\newcommand{\REMARK}[1]{\item[] \vspace{1mm} /* #1 */}

\newcommand{\our}{EPOS}
\newcommand{\ours}{\our~}

\newcommand{\rour}{Ours}
\newcommand{\rours}{\rour~}

\renewcommand{\algorithmicrequire}{\textbf{Input:}}
\renewcommand{\algorithmicensure}{\textbf{Output:}}

\renewcommand{\topfraction}{1.0}
\renewcommand{\bottomfraction}{1.0}
\renewcommand{\dbltopfraction}{1.0}
\renewcommand{\textfraction}{0.0001}
\renewcommand{\floatpagefraction}{1.0}
\renewcommand{\dblfloatpagefraction}{1.0}
\setcounter{topnumber}{100}
\setcounter{bottomnumber}{100}
\setcounter{totalnumber}{200} % http://www.ice.is.kit.ac.jp/~umehara/misc/comp/latex.html

\def\BibTeX{{\rm B\kern-.05em{\sc i\kern-.025em b}\kern-.08em T\kern-.1667em\lower.7ex\hbox{E}\kern-.125emX}}

%%% added package END %%%




\begin{document}
%
% paper title
% Titles are generally capitalized except for words such as a, an, and, as,
% at, but, by, for, in, nor, of, on, or, the, to and up, which are usually
% not capitalized unless they are the first or last word of the title.
% Linebreaks \\ can be used within to get better formatting as desired.
% Do not put math or special symbols in the title.
\title{Supplementary Material of ``An Evolutionary Algorithm Assisted by An Ensemble of Pareto-Optimal Surrogate Models''}
%
%
% author names and IEEE memberships
% note positions of commas and nonbreaking spaces ( ~ ) LaTeX will not break
% a structure at a ~ so this keeps an author's name from being broken across
% two lines.
% use \thanks{} to gain access to the first footnote area
% a separate \thanks must be used for each paragraph as LaTeX2e's \thanks
% was not built to handle multiple paragraphs
%

\author{Kei~Nishihara,~\IEEEmembership{Member,~IEEE,}
        Yaochu~Jin,~\IEEEmembership{Fellow,~IEEE,}
        and~Masaya~Nakata,~\IEEEmembership{Member,~IEEE}% <-this % stops a space

% \author{Anonymous Author(s)% <-this % stops a space

% \thanks{This work was supported by JSPS KAKENHI Grant Nos. 22KJ1409 and 20H04254. (\textit{Corresponding author: Masaya Nakata.})}% <-this % stops a space
% \thanks{K. Nishihara is with Faculty of Engineering, Yokohama National University, Kanagawa 2408501, Japan 
% (e-mail: nishihara-kei-jv@ynu.jp).}% <-this % stops a space
% \thanks{Y. Jin is with School of Engineering, Westlake University, Hangzhou 310030, China 
% (e-mail: jinyaochu@westlake.edu.cn).}% <-this % stops a space
% \thanks{M. Nakata is with Faculty of Engineering, Yokohama National University, Kanagawa 2408501, Japan 
% (e-mail: nakata-masaya-tb@ynu.ac.jp).}% <-this % stops a space

% \thanks{Manuscript received MM DD, YYYY; revised MM DD, YYYY.}

% \thanks{} \thanks{} \thanks{} \thanks{} \thanks{} \thanks{} \thanks{} \thanks{} \thanks{} \thanks{} 
}

% note the % following the last \IEEEmembership and also \thanks - 
% these prevent an unwanted space from occurring between the last author name
% and the end of the author line. i.e., if you had this:
% 
% \author{....lastname \thanks{...} \thanks{...} }
%                     ^------------^------------^----Do not want these spaces!
%
% a space would be appended to the last name and could cause every name on that
% line to be shifted left slightly. This is one of those "LaTeX things". For
% instance, "\textbf{A} \textbf{B}" will typeset as "A B" not "AB". To get
% "AB" then you have to do: "\textbf{A}\textbf{B}"
% \thanks is no different in this regard, so shield the last } of each \thanks
% that ends a line with a % and do not let a space in before the next \thanks.
% Spaces after \IEEEmembership other than the last one are OK (and needed) as
% you are supposed to have spaces between the names. For what it is worth,
% this is a minor point as most people would not even notice if the said evil
% space somehow managed to creep in.



% The paper headers
% \markboth{} 
\markboth{IEEE TRANSACTIONS ON CYBERNETICS (A preprint of the ``Accepted article'' version)}
{NISHIHARA \MakeLowercase{\textit{et al.}}: EA ASSISTED BY AN EPOS MODELS}% The only time the second header will appear is for the odd numbered pages
% after the title page when using the twoside option.
% 
% *** Note that you probably will NOT want to include the author's ***
% *** name in the headers of peer review papers.                   ***
% You can use \ifCLASSOPTIONpeerreview for conditional compilation here if
% you desire.




% If you want to put a publisher's ID mark on the page you can do it like
% this:
%\IEEEpubid{0000--0000/00\$00.00~\copyright~2015 IEEE}
% Remember, if you use this you must call \IEEEpubidadjcol in the second
% column for its text to clear the IEEEpubid mark.



% use for special paper notices
%\IEEEspecialpapernotice{(Invited Paper)}




% make the title area
\maketitle


% % As a general rule, do not put math, special symbols or citations
% % in the abstract or keywords.
% \begin{abstract}
%     An ensemble of surrogate models helps improve the prediction quality and robustness of surrogate models, and in turn, the search performance of surrogate-assisted evolutionary algorithms (SAEAs). Although different degrees of smoothness of the approximated fitness landscapes need to be carefully designed for an effective ensemble, little attention has been paid to the explicit tuning of the degree of smoothness derived by surrogate models. This study proposes an adaptive ensemble SAEA, which automatically constructs plausible ensemble models by optimizing their parameter settings. Unlike existing adaptive/ensemble SAEAs, which consider prediction accuracy alone, the proposed algorithm optimizes the structure of radial basis function networks by solving bi-objective minimization problems of approximation error and model complexity, resulting in robust ensemble models of accurate surrogate models with different degrees of smoothness of the approximated fitness landscapes. As a result, the over/under-fittings are reduced. Additionally, an infill criterion is designed so that surrogate models with different degrees of smoothness can contribute to the solution prescreening. The experimental results demonstrated the superiority of the proposed algorithm compared to the state-of-the-art SAEAs on a single-objective benchmark problem set and a real-world problem set under an expensive optimization scenario.
% \end{abstract}
    
% % Note that keywords are not normally used for peerreview papers.
% \begin{IEEEkeywords}
%     Pareto-optimal surrogate models, ensemble surrogate model, surrogate-assisted evolutionary algorithm, radial basis function network, differential evolution
% \end{IEEEkeywords}






% For peer review papers, you can put extra information on the cover
% page as needed:
% \ifCLASSOPTIONpeerreview
% \begin{center} \bfseries EDICS Category: 3-BBND \end{center}
% \fi
%
% For peerreview papers, this IEEEtran command inserts a page break and
% creates the second title. It will be ignored for other modes.
\IEEEpeerreviewmaketitle


This supplementary material supports the main manuscript entitled ``An Evolutionary Algorithm Assisted by An Ensemble of Pareto-Optimal Surrogate Models.''


\section{Additional Descriptions on DE and NSGA-II Introduced in Section~\ref{sec:tch}} \label{sec:appx-tch}


This section explains the algorithms of DE and NSGA-II in detail.


\subsection{DE: Differential Evolution} \label{sec:appx-tch-de}

The algorithm of DE is as follows. Note that the objective function is $f:\mathbb{R}^{D}\to \mathbb{R}$, $D$ is the problem dimension, and a solution is $\bm{x} =[x_{1}, \dots, x_{D}]^\mathsf{T} \in \mathbb{R}^{D}$. Let ${x}^{l}_{j}$ and ${x}^{u}_{j}$ be the lower and upper bounds for the $j$-th decision variable, respectively. 

First, DE initializes its population $\mathcal{P}=\{\bm{x}_i\}^{N}_{i=1}$ with $N$ initial solutions. Specifically, DE samples each solution $\bm{x}_i$ from a uniform distribution with a range $x_{i,j} \in [{x}^{l}_{j}, {x}^{u}_{j}]$. In the following main loop, DE repeats procedures from mutation to solution selection until the termination criteria are met.

In the mutation procedure, for each $\bm{x}_{i}$, a mutant solution $\bm{v}_{i} = [v_{i,1}, \cdots, v_{i,D}]^\mathsf{T}$ is generated using an employed mutation strategy. For example, the \textit{best/1} mutation strategy is defined as:
%
\begin{equation}
    \bm{v}_{i} = \bm{x}_{best} + F(\bm{x}_{r_1} - \bm{x}_{r_2}),
    \label{eq:best1}
\end{equation}
%
where $\bm{x}_{r_1}$ and $\bm{x}_{r_2}$ ($r_1 \neq i, r_2 \neq i$) are two mutually exclusive solutions randomly selected from $\mathcal{P}$; the best solution $\bm{x}_{best}$ has the best fitness value in $\mathcal{P}$; $F \in [0,1]$ is a scaling factor.

Then, DE produces a trial vector $\bm{u}_{i} = [u_{i,1}, \cdots, u_{i,D}]^\mathsf{T}$ for each $\bm{x}_{i}$ with a crossover strategy. A crossover rate $\mathit{CR} \in [0,1]$ is required. Following the original work, we use the \textit{binomial} crossover strategy as:
%
\begin{equation}
	u_{i,j} = 
		\begin{cases}
			v_{i,j}, & \mbox{if $rand(0,1) \leq \mathit{CR}$ or $j = j_{\mathit{rand}}$,} \\
			x_{i,j}, & \mbox{otherwise,}
		\end{cases}
	\label{eq:bin}
\end{equation}
%
where $rand(0,1)$ is a real random value in the range of $(0,1)$ sampled from a uniform distribution and $j_{\mathit{rand}}$ is an integer randomly chosen from $1$ to $D$. If the value of $u_{i,j}$ for each $i$ and $j$ exists outside the predefined range $[{x}^{l}_{j}, {x}^{u}_{j}]$, it is replaced with the nearest boundary value, i.e., ${x}^{l}_{j}$ or ${x}^{u}_{j}$.

At the end of one generation, $\bm{u}_{i}$ is evaluated and the solution selection procedure is conducted. If $f(\bm{u}_{i}) \leq f(\bm{x}_{i})$ for minimization problems, $\bm{x}_{i}$ is replaced with $\bm{u}_{i}$.


\subsection{NSGA-II: Nondominated Sorting Genetic Algorithm II} \label{sec:appx-tch-nsgaii}

The algorithm of NSGA-II is as follows. Note that this subsection assumes real-parameter bound-constrained MOPs $\bm{F}(\bm{x})=\{{f}_{1}(\bm{x}), \dots, {f}_{M}(\bm{x})\}, M\geq2, {f}_{1, \dots, M}:\mathbb{R}^D\to \mathbb{R}$. The same procedure as for DE is followed for the initialization of the population $\mathcal{P}=\{\bm{x}_i\}^{N}_{i=1}$, and the order of solutions is decided by non-dominated sorting and crowding distance (NDCD). In other words, after each solution is ranked by the number of dominated solutions, solutions of the same rank are further ranked by the crowding distance.

At every generation, NSGA-II applies Simulated Binary Crossover (SBX) and Polynomial Mutation (PM) to parent solutions selected by the tournament selection and then generates an offspring set $\mathcal{Q}$, whose size is $N$. The $j$-th decision variables of temporary offspring $\bm{o}_{1}$ and $\bm{o}_{2}$ are generated by SBX from parents $\bm{x}_{1}$ and $\bm{x}_{2}$ as:
%
\begin{align}
	&\beta = 
	\begin{cases}
	(2{r}_{j,c})^{\frac{1}{{\eta}_{c} + 1}}, & \text{if } {r}_{j,c} \leq \frac{1}{2}, \\
	\left(\frac{1}{2(1-{r}_{j,c})}\right)^{\frac{1}{{\eta}_{c} + 1}}, & \mbox{otherwise,}
	\end{cases} \nonumber\\
	&{o}_{1,j} = \frac{1}{2}\left[(1 + \beta) {x}_{1,j} + (1 - \beta) {x}_{2,j}\right], \nonumber\\
	&{o}_{2,j} = \frac{1}{2}\left[(1 - \beta) {x}_{1,j} + (1 + \beta) {x}_{2,j}\right],
	\label{eq:sbx}
\end{align}
%
where ${r}_{j,c}$ is a real random value in $(0,1)$ and ${\eta}_{c}$ is the distribution index of crossover as a hyperparameter. PM to generate offspring $\bm{u}_{i}$ whose $j$-th decision variable is ${u}_{i,j}$ for $\mathcal{Q}$ is given by:
%
\begin{align}
	&\delta = 
	\begin{cases}
	\left(\frac{2{r}_{j,m}}{1 - 2{r}_{j,m}}\right)^{\frac{1}{{\eta}_{m} + 1}} - 1, & \text{if } {r}_{j,m} \leq \frac{1}{2}, \\
	1 - \left(\frac{2(1-{r}_{j,m})}{2{r}_{j,m}}\right)^{\frac{1}{{\eta}_{m} + 1}}, & \mbox{otherwise,}
	\end{cases} \nonumber\\
	&{u}_{i,j} = {o}_{i,j} + \delta \cdot ({x}^{u}_{j} - {x}^{l}_{j}),
	\label{eq:pm}
\end{align}
%
where ${r}_{j,m}$ is a newly sampled real random value in $(0,1)$ and ${\eta}_{m}$ is the distribution index of mutation as a hyperparameter. If the value of $u_{i,j}$ for each $i$ and $j$ exists outside the predefined range $[{x}^{l}_{j}, {x}^{u}_{j}]$, it is replaced with the nearest boundary value, i.e., ${x}^{l}_{j}$ or ${x}^{u}_{j}$. Next, all solutions in $\mathcal{Q}$ are evaluated and $\mathcal{R} = \mathcal{P} \cup \mathcal{Q}$ is created. Finally, the top $N$ solutions in $\mathcal{R}$ are selected by NDCD to form $\mathcal{P}$ for the next generation.


\section{Time Complexity} \label{sec:appx-complexity}

We discuss the time complexity of \ours by comparing it with other SAEA types, i.e., normal, adaptive, and ensemble SAEAs. We assume that the number of adaptation candidates or ensemble members, i.e., ``seeds'' called in Section~\ref{sec:rtw}, is given by $N_{\mathit{cand}}$. Since the time complexity required for the model construction and prediction is dominant in SAEAs \cite{Jin2011-fd}, we focus on these processes. Let $C_{c}$ and $C_{p}$ be the time complexity for constructing one surrogate model and predicting one solution with one surrogate model, respectively. Table~\ref{tab:complexity} summarizes the time complexity of \ours compared to other SAEA types for one generation.

Normal SAEAs construct one surrogate model and predict $N$ solutions at each generation, resulting in the time complexities of $C_{c}$ and $C_{p} N$, respectively. Adaptive SAEAs construct $N_{\mathit{cand}}$ surrogate models and assess their prediction accuracy using $\mathcal{D}_{\mathit{test}}$. Then they choose one model and predict $N$ solutions at each generation. Hence, they require $(C_{c} + C_{p} |\mathcal{D}_{\mathit{test}}|)N_{\mathit{cand}}$ and $C_{p} N$ for the model construction and prediction, respectively. Ensemble SAEAs construct $N_{\mathit{cand}}$ surrogate models and predict $N$ solutions using $N_{\mathit{cand}}$ models at each generation, resulting in $C_{c} N_{\mathit{cand}}$ and $C_{p} N_{\mathit{cand}} N$, respectively. Finally, \ours constructs $N_{M} (1 + {\omega}_{\max})$ surrogate models and evaluates them using $\mathcal{D}_{\mathit{test}}$, then predicts $N$ solutions using $|\mathcal{PS}|$ models at a generation. Therefore, they require $(C_{c} + C_{p} |\mathcal{D}_{\mathit{test}}|)N_{M}(1 + {\omega}_{\max})$ and $C_{p} |\mathcal{PS}| N$ for the model construction and prediction, respectively. Considering $|\mathcal{PS}| \leq N_{M}$, $C_{p} |\mathcal{PS}| N$ can be bounded as $C_{p} N_{M} N$. 

When RBFNs are used as surrogate models, $C_{c}$ and $C_{p}$ are $O(N_{\mathit{data}}^3)$ and $O(N_{\mathit{data}})$, respectively \cite{Park1991-et}. Besides, $|\mathcal{D}_{\mathit{test}}| = \delta N_{\mathit{data}}$ is proportional to $N_{\mathit{data}}$. Thus, $C_{c} + C_{p} |\mathcal{D}_{\mathit{test}}|$ becomes $O(N_{\mathit{data}}^3 + N_{\mathit{data}}^2)$, which is dominated by $O(N_{\mathit{data}}^3)$. Accordingly, the total time complexity of each SAEA type for one generation when using RBFNs is shown in the last row of Table~\ref{tab:complexity}.

Therefore, normal SAEAs have the smallest time complexity, while the others have larger time complexities due to the multiple model constructions and/or predictions to enhance the optimization performance. Since the term with $N_{\mathit{data}}^3$ is dominant with common hyperparameter settings, if $N_{\mathit{cand}} < N_{M} {\omega}_{\max}$, \ours has the largest time complexity among all the SAEA types due to the overhead introduced by the multi-objective surrogate optimization. However, this is acceptable as long as \ours achieves better performance because the actual runtime of SAEAs is usually dominated by FEs rather than model construction and prediction \cite{Jin2001-sk,Le2013-gk,Dong2021-cs,Baldeon_Calisto2021-jn,Lu2019-om}. Nevertheless, reducing the time complexity of \ours is important, e.g., in financially expensive optimization problems. To this end, we conducted sensitivity analyses of $N_{M}$ and ${\omega}_{\max}$ in Section~\ref{sec:dis-HSA} of the Supplementary material because they are sensitive to the time complexity of \our. The results show that \ours can achieve a good balance between performance and time complexity by setting moderate values for these hyperparameters.

\begin{table*}[t]
    \renewcommand{\arraystretch}{2.3}
    \centering
    \caption{The time complexity of \ours compared to other SAEA types for one generation: Landau's O denotes examples when using RBFNs.}
    \vspace{-1mm}
    {\tabcolsep = 1mm
    \label{tab:complexity}
    \begin{minipage}[t]{0.99\textwidth}
        \centering
        \scalebox{0.925}{
            \begin{tabular}{c|c|cccc}\hline\hline
                \multicolumn{2}{c|}{}       & Normal SAEAs                                      & Adaptive SAEAs                                                        & Ensemble SAEAs                                                                        & \ours                                                                         \\\hline
                \multirow{2}{*}{\hspace{-2mm}\begin{tabular}{c} Model \\[-3mm] Construction \end{tabular}}
                        & General Notation  &	$C_{c}$	                                        &	$(C_{c} + C_{p} |\mathcal{D}_{\mathit{test}}|)N_{\mathit{cand}}$	&	$C_{c} N_{\mathit{cand}}$	                                                        &	$(C_{c} + C_{p} |\mathcal{D}_{\mathit{test}}|)N_{M}(1 + {\omega}_{\max})$   \\
                        & RBFN Case         &	$O(N_{\mathit{data}}^3)$	                    &	$O(N_{\mathit{data}}^3 N_{\mathit{cand}})$	                        &	$O(N_{\mathit{data}}^3 N_{\mathit{cand}})$	                                        &	$O(N_{\mathit{data}}^3 N_{M} {\omega}_{\max})$                              \\\hline
                \multirow{2}{*}{\hspace{-2mm}\begin{tabular}{c} Model \\[-3mm] Prediction \end{tabular}}
                        & General Notation  &	$C_{p} N$	                                    &	$C_{p} N$	                                                        &	$C_{p} N_{\mathit{cand}} N$	                                                        &	$C_{p} |\mathcal{PS}| N \leq C_{p} N_{M} N$                                 \\
                        & RBFN Case         &	$O(N_{\mathit{data}} N)$	                    &	$O(N_{\mathit{data}} N)$	                                        &	$O(N_{\mathit{data}} N_{\mathit{cand}} N)$	                                        &	$O(N_{\mathit{data}} N_{M} N)$                                              \\\hline
                Total   & RBFN Case         &	$O(N_{\mathit{data}}^3 + N_{\mathit{data}} N)$  &	$O(N_{\mathit{data}}^3 N_{\mathit{cand}} + N_{\mathit{data}} N)$    &	$O(N_{\mathit{data}}^3 N_{\mathit{cand}} + N_{\mathit{data}} N_{\mathit{cand}} N)$  &	$O(N_{\mathit{data}}^3 N_{M} {\omega}_{\max} + N_{\mathit{data}} N_{M} N)$  \\\hline
            \end{tabular}
        }
    \end{minipage}
    }
\end{table*}


\section{Hyperparameter Settings of the Compared Algorithms and \ours} \label{sec:appx-exp}

TABLE~\ref{tab:appx-hyperparams} provides hyperparameter settings of the compared algorithms and \our, where we followed the original papers for those of the compared algorithms. These settings are used in Sections~\ref{sec:exp} and \ref{sec:dis}.

\begin{table*}[t]
    \renewcommand{\arraystretch}{1.75}
    \centering
    \caption{Hyperparameter settings of the compared algorithms and the proposed algorithm (\our).}
    \label{tab:appx-hyperparams}
    % \vspace{2mm}
    \hspace{-8mm}
    \begin{minipage}[t]{0.975\textwidth}
        \centering
        \scalebox{0.9}{
            \begin{tabular}{c|l}\hline\hline
                Algorithm                       & \cth{Hyperparameter Settings} \\\hline
                \multirow{2}{*}{GL-SADE}        & ${N}_{G}\in\{100,200\}, {N}_{L}\in\{40,80\}, \mbox{ and } {\omega}_{\max}\in\{50,100\}  \mbox{ for } D\in\{30,50\&100\}, {\omega}_{\max,\mathit{RS}}=10, {|\mathcal{D}|}_{\mathit{RS}}=3D, F=0.8, \mathit{CR}=0.8,$ \\
                                                & ${L}_{1}=120, {L}_{2}=20, {\mathit{fcm}}_{1}=2, {\mathit{fcm}}_{2}=0.05, \mathit{kernel}=\mathit{cubic}, {\mathit{regression}}_{\mathit{Krg}}=\mathit{matern32}, \mathit{correlation}=\mathit{quadratic}$\\\hline
                IDRCEA                          & $N\in\{100,140,200\} \mbox{ and } \mathit{level}\in\{5,7,10\} \mbox{ for } D\in\{30,50,100\}, p=0.4, T=20, \mathit{kernel}=\mathit{cubic}, {\mathit{level}}_{\mathit{kNN}}=5, {\mathit{dist}}_{\mathit{param},\mathit{kNN}}=2$\\\hline
                \multirow{3}{*}{TS-DDEO}  & $N=50, F=0.5, \mathit{CR}_{\mathit{prescreening}}=0.5, \mathit{CR}_{\mathit{localsearch}}=0.9, {N}_{\mathit{init}}\in\{100,150\} \mbox{ for } D\in\{30\&50,100\}, {\mathit{Samp}}_{\mathit{localsearch}}=50,$ \\
                                                & ${c}_{1}={c}_{2}=2.05, {w}=0.7298, {v}_{\max}=0.5, {\mathit{FE}}_{\mathit{shift}}=300, {\mathit{Error}}_{\min}={1}^{-8}, {\omega}_{\max}=50, M=100, \beta=0.01, {m}_{\mathit{div}}=10,$ \\
                                                & ${\theta}_{\mathit{SLPSOstag}}=20, {\theta}_{\mathit{DEstag}}=10, \chi=0.25, {\theta}_{\mathit{fullcrossover}}=0.2, \mathit{kernel}=\mathit{Gaussian}$ \\\hline
                \multirow{2}{*}{MHS-QPSO} & $N\in\{5D,100\}, {N}_{\mathit{init}}\in\{N,100\}, \mbox{ and } {\omega}_{global}\in\{\max(D,20),50\} \mbox{ for } D\in\{30,50\&100\}, K=5, {\alpha}_{\mathit{QPSO}}=0.5, {K}_{\mathit{reliability}}=4,$ \\
                                                & ${\mathit{LS}}_{\mathit{datasize}}=0.2, {\mathit{LS}}_{\mathit{radius}}=0.25, \mathit{kernel}=\mathit{multi\mbox{-}quadric}$ \\\hline
                SADE-ATDSC                      & $N=100, F=0.5, \mathit{CR}=0.9, n=100, \delta=0.2, \mathit{kernel}=\mathit{cubic}$ \\\hline
                \multirow{2}{*}{AutoSAEA}       & $N=100, F=0.5, \mathit{CR}=0.9, {\mathit{FE}}_{\mathit{inner}}=100D+1000, {\mathit{Error}}_{\min}={1}^{-20}, \mathit{kernel}=\mathit{cubic}, {\mathit{regression}}_{\mathit{Krg}}=\mathit{zeroorder},$ \\
                                                & $\mathit{correlation}=\mathit{Gaussian}, \alpha=2.5, w=2, {D}_{\mathit{PR}}=2, {\mathit{regression}}_{\mathit{PR}}=\mathit{\mathit{Full}}, {\mathit{level}}_{\mathit{kNN}}=5, {\mathit{dist}}_{\mathit{param},\mathit{kNN}}=2$ \\\hline
                \multirow{2}{*}{CAL-SAPSO}      & $N=50, {c}_{1}={c}_{2}=1.49445, {w}_{1}=0.9, {w}_{2}=0.5, {v}_{\max}=0.5, {N}_{\mathit{init}}=5D, {g}_{\max}=100, {D}_{\mathit{norm}}=2, \mathit{kernel}=\mathit{multi\mbox{-}quadric},$ \\
                                                & ${\mathit{regression}}_{\mathit{Krg}}=\mathit{zeroorder}, \mathit{correlation}=\mathit{Gaussian}, \theta_{\mathit{init}}={|\mathcal{D}_{\mathit{train}}|}^{-\frac{1}{D}}, {D}_{\mathit{PR}}=2, {\mathit{regression}}_{\mathit{PR}}=\mathit{\mathit{Full}}$\\\hline
                \multirow{3}{*}{EAPSO}          & $N=60, {N}_{\min}=3D, {N}_{\mathit{init}}=100, {c}_{1}={c}_{2}=1.491, {w}_{1}=0.729, {w}_{2}=0.4, {v}_{\max}=0.25, {v}_{\mathit{init}}=0.15, r = 10, {\alpha}_{\mathit{init}}=0.5, {\omega}_{\mathit{damp}}=0.995,$ \\
                                                & $\mathit{div}=4, {\theta}_{\mathit{local}}=0.75, {N}_{\mathit{local}}=10, {d}_{\mathit{limit}}=0.001, \mathit{kernel}=\mathit{bi\mbox{-}harmonic \& inverse\mbox{-}multi\mbox{-}quadric}, {\mathit{RBFN}}_{\mathit{poly}}=1.0002,$ \\
                                                & ${\mathit{FE}}_{\mathit{inner}}=3000, {\mathit{Error}}_{\min}={1}^{-8}, {D}_{\mathit{PR}}=2, {\mathit{regression}}_{\mathit{PR}}=\mathit{\mathit{Full}}$\\\hline
                HESNFO                          & $N=100, F=1.3, \mathit{CR}=0.9, {N}_{\mathit{init}}=5D, \delta=0.5, {d}_{\mathit{limit}}=0.01, |V|= 2$ \\\hline
                \multirow{3}{*}{DSP-SAEA}       & $N=5D, k=5, \omega=7, {\theta}_{D1}=50, {\theta}_{D2}=5D, {\theta}_{P}=5D, {d}_{\mathit{limit},\mathit{CSOGP},1}=0.001, {d}_{\mathit{limit},\mathit{CSOGP},2}=0.01, {N}_{\mathit{YCSO}}=50, {\omega}_{\mathit{YCSO}}=100,$ \\
                                                & ${\phi}_{\mathit{YCSO}}=1, es=\{1, 2\}, \rho=\{0.25, 0.75\}, {d}_{\mathit{limit},\mathit{CSOLRA}}=0.001, {N}_{\mathit{CSOLRA}}=50, {\omega}_{\mathit{CSOLRA}}=100, {\phi}_{\mathit{CSOLRA}}=1, {\delta}_{\mathit{CSOLRA}}=0.2,$ \\
                                                & ${\mathit{Error}}_{\min}={1}^{-20}, \mathit{kernel}=\mathit{cubic}, {\mathit{regression}}_{\mathit{Krg}}=\mathit{zeroorder}, \mathit{correlation}=\mathit{Gaussian}, \theta_{\mathit{init}}={|\mathcal{D}_{\mathit{train}}|}^{-\frac{1}{D}}, {D}_{\mathit{PR}}=2, {\mathit{regression}}_{\mathit{PR}}=\mathit{\mathit{Full}}$ \\\hline
                \ours                           & $N=100, F=0.5, \mathit{CR}=0.9, {N}_{\mathit{data}}=5D, \delta=0.2, {N}_{\mathit{M}}=10, {\omega}_{\max}=10, {\eta}_{c}=20, {\eta}_{m}=20, \alpha=2, \mathit{kernel}=\mathit{Gaussian}$ \\\hline
            \end{tabular}
        }
    \end{minipage}
\end{table*}


\section{The Detailed Results Obtained in the Experiments in Section~\ref{sec:exp}} \label{sec:appx-expAdd}

\subsection{Additional Results} \label{sec:appx-expAdd-ar}

TABLE~\ref{tab:data_move2appx} provides the detailed results of the average fitness values and standard deviations (in parentheses) obtained at $1,000$ FEs for $D \in \{30,50,100\}$ in Section~\ref{sec:exp}. The best and worst values among the eleven algorithms are highlighted in green bold and pink italics, respectively. The summary of these results shown at the bottom of TABLE~\ref{tab:data_move2appx} is identical to the contents of TABLE~\ref{tab:data_summary} in Section~\ref{sec:exp}.

Fig.~\ref{fig:convergence_curve} shows the convergence curves of the performance of the compared algorithms and \ours obtained in the experiments in Section~\ref{sec:exp}. The vertical axes showing objective function values employ logarithmic scales.

\subsection{Discussion on the Results in Section~\ref{sec:exp} from the Point of View of the Difference in Adaptation/Ensemble Methods} \label{sec:appx-expAdd-dis}

Next, we discuss the results from the point of view of the difference in adaptation/ensemble methods. For SAEAs with adaptation mechanisms, while SADE-ATDSC, AutoSAEA, HESNFO, and DSP-SAEA have four, eight, five, and four adaptation candidates, respectively, \ours has $110$ candidates. Considering the superiority of the performance of \our, the variety of adaptation candidates contributed to the performance improvement in SAEAs with adaptation mechanisms. Since \ours significantly outperformed SADE-ATDSC, HESNFO, and DSP-SAEA, the surrogate model complexity should also be considered in the adaptation in SAEAs. This also suggests that selecting surrogate models based on approximation error alone may make a surrogate selection method highly problem-dependent. In comparison with SADE-ATDSC or AutoSAEA, the number of ``$-$'' increased as the problem dimension increased. This indicates that the use of less complex surrogate models in the ensemble mechanism of \ours can cope with the increase in the difficulty of higher dimensionality. This implies that smooth surrogate models in the Pareto set of \ours can capture the entire landscape and contribute to improving performance with a small number of FEs, whereas enhancing the performance of reinforcement learning in AutoSAEA requires a large number of samples (FEs) with high-dimensional cases. For ensemble SAEAs, \ours outperformed CAL-SAPSO and EAPSO for most problems and all problem dimensions although EAPSO uses the same infill criterion, i.e., LCB, which suggests that the degree of smoothness of the approximated fitness landscapes derived by surrogate models should be finely controlled for the ensemble. Even if both adaptation and ensemble mechanisms are employed in HESNFO and DSP-SAEA, the multi-objective optimization of surrogate models in \ours was more useful in generating various surrogate models effective for the ensemble.


\section{Algorithm of the Variant of \ours Used in Section~\ref{sec:dis-MOP}} \label{sec:appx-disMOP}

This section shows a pseudo-code of the variant of \our, which is proposed to evaluate the effectiveness of multi-objectivization in the surrogate model adaptation of \ours in Section~\ref{sec:dis-MOP}. Unlike \our, the varinat considers only the approximation accuracy or simplicity of surrogate models in the surrogate model adaptation, whose pseudo-code is given in Algorithm~\ref{alg:appx-soea}, where the changes from Algorithm~\ref{alg:our} are underlined.

\begin{algorithm}[h]
    \caption{A Variant of \ours with Single-objective Optimization of Surrogate Models} \label{alg:appx-soea}
    \small
	\begin{algorithmic}[1]
        \REQUIRE the maximum number of function evaluations $\mathit{FE}_{\max}$, population size $N$, scaling factor for DE $F$, crossover rate for DE $\mathit{CR}$, data size for surrogate modeling $N_{\mathit{data}}$, test-data rate $\delta$, population size for GA $N_M$, the maximum number of generations for GA ${\omega}_{\max}$, distribution index of crossover for GA ${\eta}_{c}$, and distribution index of mutation for GA ${\eta}_{m}$
		\STATE Initialize $\hspace{-2pt}\mathcal{P}\hspace{-2pt}=\hspace{-2pt}\{\bm{x}_{i}\}_{i=1}^{N}\hspace{-2pt}$ by LHS and Evaluate $\forall \bm{x} \hspace{-2pt}\in\hspace{-2pt} \mathcal{P}$ with true $f$
		\STATE $\mathcal{A} = \{\left(\bm{x}_{i}, f(\bm{x}_{i})\right)\}_{i=1}^{N}$, $\mathit{FE}=N$
		\WHILE{$\mathit{FE}<\mathit{FE}_{\max}$}
            \REMARK{\textbf{Phase 1}: Adaptation of Surrogate Models}
            \STATE $\mathcal{D} \gets$ Get top $N_{\mathit{data}}$ data from $\mathcal{A}$
            \STATE Divide $\mathcal{D}$ into training/test datasets in the ratio $(1-\delta):\delta$
            \STATE Set the GA boundary \hfill | Eqs.~(\ref{eq:MOP_x1})\&(\ref{eq:MOP_x2}) \label{alg-l:MOEA-begin}
            \STATE Initialize $\mathcal{P}_{\mathit{M}}=\{\bm{x}_{\mathit{M},i}\}_{i=1}^{{N}_{\mathit{M}}}$ by LHS
            \STATE Construct RBFNs $\forall \bm{x}_{M} \in \mathcal{P}_{M}$ and Evaluate
            \STATE \uline{Sort $\mathcal{P}_{\mathit{M}}$ in terms of the objective} \label{alg-l:sort1}
            \vspace{1mm}
            \FOR{$\omega=1$ \TO ${\omega}_{\max}$}
                \STATE $\mathcal{Q}_{M} \gets$ Generate ${N}_{M}$ offspring from $\mathcal{P}_{M}$ with ${\eta}_{c}$ \& ${\eta}_{m}$
                \STATE Construct RBFNs $\forall \bm{x}_{M} \in \mathcal{P}_{M}$ and Evaluate
                \STATE \uline{Sort $\mathcal{R}_{\mathit{M}}=\mathcal{P}_{\mathit{M}}\cup\mathcal{Q}_{\mathit{M}}$ in terms of the objective} \label{alg-l:sort2}
                \vspace{1mm}
                \STATE $\mathcal{P}_{M} \gets$ Select top ${N}_{M}$ solutions from $\mathcal{R}_{M}$
            \ENDFOR

            \REMARK{\textbf{Phase 2}: Offspring Generation by DE}
            \STATE $\mathcal{P} \gets$ Get top $N$ solutions from $\mathcal{A}$
            \STATE $\mathcal{Q} \gets$ Generate $N$ offspring from $\mathcal{P}$ with $F$ \& $\mathit{CR}$
                \\ \hfill | Eqs.~(\ref{eq:best1})\&(\ref{eq:bin})

            \REMARK{\textbf{Phase 3}: Prescreening of Offspring} 
            \STATE \uline{Select the best surrogate model $\hat{f}$ in $\mathcal{P}_{\mathit{M}}$} \label{alg-l:prescreening}
            \vspace{1mm}
            \STATE \uline{$\bm{u}^{*} \gets \argmin_{\bm{u}\in\mathcal{Q}} \hat{f}(\bm{u})$} 
            \vspace{1mm}
            \STATE $f(\bm{u}^{*}) \gets$ Evaluate $\bm{u}^{*}$ with true $f$
            \STATE $\mathcal{A} = \mathcal{A} \cup \{(\bm{u}^{*}, f(\bm{u}^{*}))\}$, $\mathit{FE}=\mathit{FE}+1$ 
		\ENDWHILE
        \ENSURE The best solution in $\mathcal{A}$
	\end{algorithmic}
\end{algorithm}


\section{The Detailed Results Obtained in the Real-world Application} \label{sec:appx-disRW}

This section adds the average fitness values and standard deviations to TABLE~\ref{tab:data_CEC2011RW} in Section~\ref{sec:dis-RW}. TABLE~\ref{tab:appx-data_CEC2011RW} lists these values obtained at $1,000$ FEs in addition to the contents of TABLE~\ref{tab:data_CEC2011RW}, i.e., the results of the Wilcoxon signed-rank test with a significance level of $0.05$ and average rank. The best and worst fitness values among eleven algorithms are highlighted in green bold and pink italics, respectively. The statistical test results are reported with ``$+$,'' ``$-$,'' or ``$\sim$,'' indicating that the compared algorithm significantly outperformed \our, significantly underperformed \our, or we cannot find a significant difference, respectively.

Fig.~\ref{fig:convergence_curve_CEC2011RW} summarizes the convergence curves of the performance of the compared algorithms and \ours obtained in this real-world application.


\section{Comparison of the Search Strategies} \label{sec:appx-disIterative}

\ours employs the prescreening strategy instead of the iterative search strategy. This section validates its effect by comparing the optimization performance on the \ours framework. The variant procedure using iterative search is shown in Algorithm~\ref{alg:our_iterative}, which is a modification of Algorithm~\ref{alg:our}. The changes from Algorithm~\ref{alg:our} to Algorithm~\ref{alg:our_iterative} are highlighted with underlines. The newly added hyperparameter, the maximum number of generations for DE in the iterative search ${\omega}_{\max,\mathit{DE}}$, was set to ${\omega}_{\max,\mathit{DE}}=30$ according to \cite{Pan2021-jj}. That is, this variant conducts the iterative search for ${\omega}_{\max,\mathit{DE}}$ generations to obtain a solution for the function evaluation via an intensive search using an acquisition function. The experimental settings are identical to Section~\ref{sec:exp}.

Table~\ref{tab:sigs_iterative} summarizes the comparison results at $1,000$ fitness evaluations. The test results of the Wilcoxon signed-rank test are reported with ``$+$,'' ``$-$,'' or ``$\sim$,'' which stands for the variant significantly outperformed, significantly underperformed, or was competitive to the original \our, respectively. From the table, we can confirm that the original \ours outperformed the variants. Specifically, the performance of \ours was superior to the variants with statistically significant differences on $28$ problem instances out of $30$. It is worth mentioning that the prescreening was effective in all the cases with $D \in \{50,100\}$. This happend because the prescreening strategy was able to maintain the diversity of the evaluated solution due to its shallow search, which contributed to constructing more promising ensemble surrogate models than the highly exploiting iterative search.

\begin{algorithm}[t]
    \caption{A Variant of \ours That Conducts The Iterative Search Using The Acquisition Function Instead of The Prescreening} \label{alg:our_iterative}
    \small
    \begin{algorithmic}[1]
        \REQUIRE the maximum number of function evaluations $\mathit{FE}_{\max}$, population size $N$, scaling factor for DE $F$, crossover rate for DE $\mathit{CR}$, data size for surrogate modeling $N_{\mathit{data}}$, test-data rate $\delta$, population size for NSGA-II $N_M$, the maximum number of generations for NSGA-II ${\omega}_{\max}$, distribution index of crossover for NSGA-II ${\eta}_{c}$, distribution index of mutation for NSGA-II ${\eta}_{m}$, coefficient of LCB $\alpha$, \uline{and the maximum number of generations for DE ${\omega}_{\max,\mathit{DE}}$}
        \STATE Initialize $\hspace{-2pt}\mathcal{P}\hspace{-2pt}=\hspace{-2pt}\{\bm{x}_{i}\}_{i=1}^{N}\hspace{-2pt}$ by LHS and Evaluate $\forall \bm{x} \hspace{-2pt}\in\hspace{-2pt} \mathcal{P}$ with true $f$
        \STATE $\mathcal{A} = \{\left(\bm{x}_{i}, f(\bm{x}_{i})\right)\}_{i=1}^{N}$, $\mathit{FE}=N$
        \WHILE{$\mathit{FE}<\mathit{FE}_{\max}$}
            \REMARK{\textbf{Phase 1}: Adaptation of Surrogate Models}
            \STATE $\mathcal{D} \gets$ Get top $N_{\mathit{data}}$ data from $\mathcal{A}$
            \STATE Divide $\mathcal{D}$ into training/test datasets in the ratio $(1-\delta):\delta$
            \STATE Set the NSGA-II boundary \hfill | Eqs.~(\ref{eq:MOP_x1})\&(\ref{eq:MOP_x2})
            \STATE Initialize $\mathcal{P}_{M}=\{\bm{x}_{M,i}\}_{i=1}^{{N}_{M}}$ by LHS
            \STATE Construct RBFNs $\forall \bm{x}_{M} \in \mathcal{P}_{M}$ and Evaluate \hfill | Eq.~(\ref{eq:MOP})
            \STATE Perform NDCD on $\mathcal{P}_{M}$
            \FOR{$\omega=1$ \TO ${\omega}_{\max}$}
                \STATE $\mathcal{Q}_{M} \gets$ Generate ${N}_{M}$ offspring from $\mathcal{P}_{M}$ with ${\eta}_{c}$ \& ${\eta}_{m}$
                    \\ \hfill | Eqs.~(\ref{eq:sbx})\&(\ref{eq:pm})
                \STATE Construct RBFNs $\forall \bm{x}_{M} \in \mathcal{P}_{M}$ and Evaluate \hfill | Eq.~(\ref{eq:MOP})
                \STATE Perform NDCD on $\mathcal{R}_{M}=\mathcal{P}_{M}\cup\mathcal{Q}_{M}$
                \STATE $\mathcal{P}_{M} \gets$ Select top ${N}_{M}$ solutions from $\mathcal{R}_{M}$
            \ENDFOR
            \STATE $\mathcal{PS} \gets$ Get a Pareto set from $\mathcal{P}_{M}$

            \REMARK{\textbf{Phase 2}: \uline{Iterative Search Using Acquisition Function}}
            \STATE \uline{Construct an ensemble model of all in $\mathcal{PS}$} \hfill | Eqs.~(\ref{eq:mean})\&(\ref{eq:sd})
            \STATE \uline{Initialize $\mathcal{P}=\{\bm{x}_{i}\}_{i=1}^{N}$ by LHS}
            \FOR{$\omega=1$ \TO ${\omega}_{\max,\mathit{DE}}$} 
                \STATE \uline{$\mathcal{Q} \gets$ Generate $N$ offspring from $\mathcal{P}$ with $F$ \& $\mathit{CR}$
                \\ \hfill | Eqs.~(\ref{eq:best1})\&(\ref{eq:bin})}
                \FOR{$i=1$ \TO $N$} 
                    \STATE \uline{Replace $\bm{x}_{i} \in \mathcal{P}$ with $\bm{u}_{i} \in \mathcal{Q}$ if $\mathit{LCB}(\bm{u}_{i}) \leq \mathit{LCB}(\bm{x}_{i})$, where $\mathit{LCB}(\cdot)$ is calculated with $\alpha$} \hfill | Eq.~(\ref{eq:LCB})
                \ENDFOR
            \ENDFOR

            \STATE \uline{$\bm{u}^{*} \gets \argmin_{\bm{u}\in\mathcal{P}} \mathit{LCB}(\bm{u})$}
            \STATE $f(\bm{u}^{*}) \gets$ Evaluate $\bm{u}^{*}$ with true $f$
            \STATE $\mathcal{A} = \mathcal{A} \cup \{(\bm{u}^{*}, f(\bm{u}^{*}))\}$, $\mathit{FE}=\mathit{FE}+1$
        \ENDWHILE
        \ENSURE The best solution in $\mathcal{A}$
    \end{algorithmic}
\end{algorithm}

\begin{table}[t]
    \renewcommand{\arraystretch}{1.5}
    \centering
    \caption{The summary of results at $1,000$ fitness evaluations obtained in the comparison between the original \ours and its variant that conducts the iterative search using the acquisition function instead of the prescreening.}
    \vspace{-1mm}
    {\tabcolsep = 1.5mm
    \label{tab:sigs_iterative}
    \begin{minipage}[t]{0.495\textwidth}
        \centering
        \scalebox{1}{
            \begin{tabular}{c|ccccccccccc}\hline\hline
                 & Iterative Search & Prescreening (The Original \our) \\\hline
                $+/-/\sim$	&		2/28/0		&		-	\\
                Ave. Rank	&	\worst	1.933 		&	\win	1.067 	\\ \hline
            \end{tabular}
        }
    \end{minipage}
    }
\end{table}


\section{Sensitivity Analysis of Hyperparameters of Surrogate Model Construction} \label{sec:dis-HSA}

We conducted sensitivity analysis of the hyperparameters used in the multi-objective adaptation of surrogate models, i.e., the population size of NSGA-II ${N}_{M}$ and the maximum number of generations ${\omega}_{\max}$, where the number of total surrogate models constructed in a generation is calculated by ${N}_{M} + {N}_{M} \times {\omega}_{\max}$. For both hyperparameters, we used the values of $\{5, 10, 15\}$, thus $3 \times 3 = 9$ settings were tested, where ${N}_{M}={\omega}_{\max}=10$ is the default setting.

TABLE~\ref{tab:summary_HSA} summarizes the hyperparameter settings, the total number of constructed surrogate models, the summary of Wilcoxon signed-rank test results, the average rank, and the average computational times [sec] for $D\in\{30,50,100\}$. The signs in the statistical test, ``$+$,'' ``$-$,'' and ``$\sim$'' correspond to the significant superiority, significant inferiority, and competitiveness, respectively, of \ours with various hyperparameter settings to that with the default settings (${N}_{M}={\omega}_{\max}=10$). From the table, the smaller settings, i.e., $\{{N}_{M}, {\omega}_{\max}\}\in\{\{5,5\},\{5,10\},\{10,5\}\}$, were inappropriate because the only small number of surrogate models were constructed and they were not adequately optimized, resulting in their statistically low performance and the lower average ranks. \ours with the middle values of hyperparameter settings ($\{{N}_{M}, {\omega}_{\max}\}\in\{\{5,15\},\{10,10\},\{15,5\}\}$) obtained the highest average ranks as well as the moderate computational time. Finally, when ${N}_{M}$ and ${\omega}_{\max}$ increased to $\{{N}_{M}, {\omega}_{\max}\}\in\{\{10,15\},\{15,10\},\{15,15\}\}$, the computational time became significantly larger to construct many surrogate models, while the performance of variants was competitive to that of the default in the statistical test, and their average ranks slightly deteriorated. Taking into account the balance between satisfying performance and realistic computational time, the moderate number of surrogate models, i.e., from $80$ to $110$, was suitable.

\begin{table*}[t]
    \renewcommand{\arraystretch}{1.75}
    \centering
    \caption{The summary of results at $1,000$ fitness evaluations obtained in the sensitivity analysis of the hyperparameters of surrogate model construction.}
    \vspace{-2mm}
    % {\tabcolsep = 1.2mm
    \label{tab:summary_HSA}
    \begin{minipage}[t]{0.995\textwidth}
        \centering
        \scalebox{0.95}{
            \begin{tabular}{c|ccccccccccc}\hline\hline
                ${N}_{M}$                               &       5           &       5           &       5           &       10          &       10          &       15          &       15          &       15          &       10 (default)\\
                ${\omega}_{\max}$                       &       5           &       10          &       15          &       5           &       15          &       5           &       10          &       15          &       10 (default)\\
                ${N}_{M}+{N}_{M}\times{\omega}_{\max}$  &       30          &       55          &       80          &       60          &       160         &       90          &       165         &       240         &       110         \\ \hline
                $+/-/\sim$		                        &		2/11/17		&		0/6/24		&		1/3/26		&		0/4/26		&		0/0/30		&		0/1/29		&		0/0/30		&		1/0/29		&		-	        \\
                Ave. Rank		                        & \worst 6.000 		&		5.967 		& \win	4.333 		&		5.333 		&		4.667 		&		4.433 		&		4.933 		&		4.733 		&		4.600 	    \\ \hline
                Comput. Time ($D=30$)\;\;               & 1.232E+03	        & 2.137E+03	        & 2.755E+03	        & 3.199E+03	        & 7.249E+03	        & 4.114E+03	        & 7.266E+03	        & 1.016E+04	        & 4.737E+03         \\
                Comput. Time ($D=50$)\;\;               & 1.609E+03	        & 2.828E+03	        & 3.750E+03	        & 3.848E+03	        & 9.320E+03	        & 5.253E+03	        & 9.339E+03	        & 1.287E+04	        & 6.124E+03         \\
                Comput. Time ($D=100$)                  & 2.439E+03	        & 4.118E+03	        & 5.176E+03	        & 6.380E+03	        & 1.362E+04	        & 8.618E+03	        & 1.292E+04	        & 2.073E+04	        & 9.573E+03         \\ \hline
            \end{tabular}
            }
        \end{minipage}
        % }
        \vspace{-2mm}
\end{table*}



\section{Sensitivity Analysis of Hyperparameters of Evolutionary Optimization} \label{sec:dis-HSA2}

We conducted a sensitivity analysis of the hyperparameters of DE, i.e., the scaling parameter $F$ and the crossover rate $\mathit{CR}$. These hyperparameters directly affect the solution generation process to be evaluated. Specifically, we used $F\in\{0.2, 0.5 \ \mbox{(default)}, 0.8\}$ and $\mathit{CR}\in\{0.5, 0.9 \ \mbox{(default)}, 1.0\}$. Considering every pair, we tested nine pairs in total including the default settings of $F=0.5$ and $\mathit{CR}=0.9$.

TABLE~\ref{tab:summary_HSA2} provides the summary of results comprising the hyperparameter settings, Wilcoxon signed-rank test results, and average rank for $D\in\{30,50,100\}$. The test results are demonstrated with signs of  ``$+$,'' ``$-$,'' and ``$\sim$,'' indicating the significant superiority, significant inferiority, and competitiveness, respectively, of \ours with different hyperparameter settings to that with the default settings. The table demonstrates that both hyperparameters of DE were sensitive to the performance of \our. Regarding $F$, the default setting of $F=0.5$ was highly competitive to $F=0.2$ and statistically outperformed $F=0.8$ under the same setting of $\mathit{CR}=0.9$, whose results were $+/-/\sim=3/9/18$ and $0/28/2$, respectively. This may be because we employed the \textit{best/1} mutation strategy. Specifically, the small value of $F$ caused premature convergence while the larger value decreased the convergence speed due to long difference vectors. A similar tendency was observed with different values of $\mathit{CR}$. Notably, $F=0.8$ was inappropriate because they statistically underperformed $F=0.5$ and obtained lower average ranks. As for $\mathit{CR}$, we should avoid $\mathit{CR}=1.0$ because it underperformed $\mathit{CR}=0.9$ on $27$, $24$, and $26$ problem instances out of $30$ with $F=0.2, 0.5,$ and $0.8$, respectively. This may be because the setting of $\mathit{CR}=1.0$ does not enjoy the benefit of the current best solution. Conversely, $\mathit{CR}=0.5$ utilizes too many dimensions of the current best solution, which prevents the evolutionary search, resulting in slightly poor performance than the default settings, i.e., $\mathit{CR}=0.9$.


\begin{table*}[t]
    \renewcommand{\arraystretch}{1.75}
    \centering
    \caption{The summary of results at $1,000$ fitness evaluations obtained in the sensitivity analysis of the hyperparameters of evolutionary optimization.}
    \vspace{-2mm}
    % {\tabcolsep = 1.2mm
    \label{tab:summary_HSA2}
    \begin{minipage}[t]{0.995\textwidth}
        \centering
        \scalebox{0.95}{
            \begin{tabular}{c|ccccccccccc}\hline\hline
                $F$             &       0.2         &       0.2         &       0.2         &       0.5         &       0.5         &       0.8         &       0.8         &       0.8         &       0.5 (default)   \\
                $\mathit{CR}$   &       0.5         &       0.9         &       1.0         &       0.5         &       1.0         &       0.5         &       0.9         &       1.0         &       0.9 (default)   \\ \hline
                $+/-/\sim$		&		3/18/9	    &       3/9/18	    &       3/27/0	    &       6/10/14	    &       4/24/2	    &       1/25/4	    &       0/28/2	    &       0/26/4      &		-	            \\
                Ave. Rank		&       4.500 	    &       3.300 	    &       6.833 	    &       2.633 	    &       6.000 	    &       6.167 	    &       5.567 	    & \worst 7.533 	    & \win  2.467           \\ \hline
            \end{tabular}
        }
    \end{minipage}
        % }
        \vspace{-2mm}
\end{table*}



\section{Effect of the Ensemble Size on the Performance} \label{sec:dis-ensemblesize}

The original \ours uses all surrogate models in the Pareto set $\mathcal{PS}$ to construct an ensemble model as shown in Line~\ref{alg-l:prescreening-begin} of Algorithm~\ref{alg:our}. In particular, ${N}_{M}=10$ models are used at maximum. We call the number of surrogate models used for the ensemble ``the ensemble size.'' However, using all surrogate models in $\mathcal{PS}$ may be redundant if better ensemble models can be constructed with a small ensemble size. Then, we prepared some variants of \ours with small ensemble sizes and observed their effect on the performance of \our. Specifically, the variants select a certain number of surrogate models from $\mathcal{PS}$ by NDCD (see Section~\ref{sec:appx-tch-nsgaii}) and then construct an ensemble model using the selected models. We set the ensemble size to $\{2,4,7,10\mbox{ (default)}\}$. The setting of two is an extreme case because the most accurate surrogate model and the least complex one are used for the ensemble. The experimental design is identical to the main experiment.

TABLE~\ref{tab:sigs_ensemblesize} is a highlight of the results at $1,000$ FEs for $D \in \{30,50,100\}$. The results of the Wilcoxon signed-rank test are reported with ``$+$,'' ``$-$,'' or ``$\sim$,'' which stands for the significant superiority, significant inferiority, or competitiveness, respectively, of \ours with different ensemble size to that of the default setting. In the table, the ensemble size of two was inappropriate, judging from the statistical result. This is because an ensemble model with only extreme models lacks the robustness of the performance. Since these extreme models have quite different characteristics, the constructed ensemble model could not merge their strong points under the complex benchmark problems. Additionally, the average model and emulated LCB are highly sensitive to these extreme models. Thus, if \ours fails in obtaining good models, the quality of the ensemble model also deteriorates with fewer surrogate models. When the performance of \ours with the ensemble size of four or seven was compared, \ours with the default setting derived the least number of worst fitness values in the $30$ experimental cases. This resulted in the best average rank of \ours although we cannot find statistical significance. Consequently, we use all the surrogate models in the Pareto set $\mathcal{PS}$ to avoid unwanted failures.

\begin{table}[t]
    \renewcommand{\arraystretch}{1.5}
    \centering
    \caption{The summary of results at $1,000$ fitness evaluations obtained in the ablation study on ensemble size.}
    \vspace{-1mm}
    % {\tabcolsep = 1.5mm
    \label{tab:sigs_ensemblesize}
    \begin{minipage}[t]{0.495\textwidth}
        \centering
        \scalebox{1}{
            \begin{tabular}{c|ccccccccccc}\hline\hline
                 & size 2 & size 4 & size 7 & all (default)\\\hline
                $+/-/\sim$	&		0/4/26		&		0/0/30		&		0/0/30		&		-	\\ 
                Ave. Rank	&		2.600 		&		2.467 		&	\worst	2.700 		&	\win	2.233 	\\ \hline
            \end{tabular}
        }
    \end{minipage}
    % }

\end{table}




\begin{table*}[t]
    \renewcommand{\arraystretch}{1.4}
    \centering
    \caption{The average fitness values discovered at $1,000$ fitness evaluations for $D \in \{30,50,100\}$ on the CEC2020 Benchmark Suite.}
    % \vspace{1mm}
    \label{tab:data_move2appx}
    \centering
    \scalebox{0.75}{
        \begin{tabular}{l|r|cccc|cc|cc|ccc}\hline\hline
                                &							& \multicolumn{4}{c|}{Normal SAEAs}                                                                                                                 & \multicolumn{2}{c|}{Adaptive SAEAs}                                   & \multicolumn{2}{c|}{Ensemble SAEAs}                               & \multicolumn{3}{c}{Adaptive Ensemble SAEAs}                                                       \\
            ID                  &	\multicolumn{1}{c|}{$D$}& GL-SADE                           & IDRCEA                            & TS-DDEO                               & MHS-QPSO                          & SADE-ATDSC                        & AutoSAEA                          & CAL-SAPSO                         & EAPSO                         & HESNFO                            & DSP-SAEA                          & \ours                     \\\hline
            \multirow{6}{*}{F1} &	\multirow{2}{*}{30}		&	    	4.450e$+$09 	\minus	&	\worst	6.435e$+$10 	\minus	&	       	2.016e$+$03 	\plus	    &	   	1.723e$+$05 	\minus	    &		    2.348e$+$08 	\nodiff	&		    8.461e$+$04 	\minus	&		1.630e$+$09 	\minus	    &		1.293e$+$10 	\minus	&		    2.123e$+$10 	\minus	&	\win	1.846e$+$03 	\plus	&		    4.696e$+$03 	\\
                                &                           &	    	(2.939e$+$09) 		    &	\worst	(1.446e$+$10) 		    &	       	(1.980e$+$03) 		        &	   	(6.394e$+$05) 		        &		    (1.132e$+$09) 		    &		    (7.032e$+$04) 		    &		(7.779e$+$08) 		        &		(3.458e$+$09) 		    &		    (8.378e$+$09) 		    &	\win	(9.934e$+$02) 		    &		    (2.637e$+$03) 	\\
                                &	\multirow{2}{*}{50}		&	    	5.920e$+$09 	\minus	&	\worst	1.659e$+$11 	\minus	&	   \win	1.026e$+$06 	\plus	    &	   	4.737e$+$07 	\minus	    &		    2.290e$+$08 	\minus	&		    1.992e$+$08 	\minus	&		1.805e$+$09 	\minus	    &		3.815e$+$10 	\minus	&		    7.306e$+$10 	\minus	&		    1.782e$+$07 	\minus	&		    6.453e$+$06 	\\
                                &                           &	    	(3.471e$+$09) 		    &	\worst	(1.534e$+$10) 		    &	   \win	(5.118e$+$06) 		        &	   	(2.629e$+$08) 		        &		    (6.362e$+$08) 		    &		    (1.142e$+$08) 		    &		(6.610e$+$08) 		        &		(7.037e$+$09) 		    &		    (1.682e$+$10) 		    &		    (5.521e$+$06) 		    &		    (3.306e$+$06) 	\\
                                &	\multirow{2}{*}{100}	&	    	1.036e$+$10 	\minus	&	\worst	4.760e$+$11 	\minus	&	   \win	1.274e$+$08 	\plus	    &	   	1.792e$+$10 	\nodiff	    &		    8.838e$+$09 	\minus	&		    8.312e$+$10 	\minus	&		3.210e$+$10 	\minus	    &		1.419e$+$11 	\minus	&		    4.021e$+$11 	\minus	&		    7.590e$+$09 	\minus	&		    3.969e$+$09 	\\
                                &                           &	    	(5.010e$+$09) 		    &	\worst	(3.042e$+$10) 		    &	   \win	(8.517e$+$07) 		        &	   	(2.834e$+$10) 		        &		    (2.792e$+$09) 		    &		    (1.504e$+$10) 		    &		(3.482e$+$09) 		        &		(1.320e$+$10) 		    &		    (9.163e$+$10) 		    &		    (1.341e$+$09) 		    &		    (1.268e$+$09) 	\\ \hline
            \multirow{6}{*}{F2} &	\multirow{2}{*}{30}		&	    	6.197e$+$03 	\minus	&	    	8.365e$+$03 	\minus	&	       	8.338e$+$03 	\minus	    &	   	6.011e$+$03 	\minus	    &		    6.688e$+$03 	\minus	&		    8.239e$+$03 	\minus	&		5.450e$+$03 	\minus	    &		6.883e$+$03 	\minus	&	\worst	8.556e$+$03 	\minus	&		    5.988e$+$03 	\minus	&	\win	4.379e$+$03 	\\
                                &                           &	    	(1.624e$+$03) 		    &	    	(3.422e$+$02) 		    &	       	(5.100e$+$02) 		        &	   	(1.566e$+$03) 		        &		    (1.943e$+$03) 		    &		    (1.007e$+$03) 		    &		(1.672e$+$03) 		        &		(9.015e$+$02) 		    &	\worst	(3.747e$+$02) 		    &		    (1.473e$+$03) 		    &	\win	(8.739e$+$02) 	\\
                                &	\multirow{2}{*}{50}		&	    	1.513e$+$04 	\minus	&	    	1.537e$+$04 	\minus	&	 \worst	1.558e$+$04 	\minus	    &	   	1.355e$+$04 	\minus	    &		    1.069e$+$04 	\minus	&		    1.547e$+$04 	\minus	&		1.412e$+$04 	\minus	    &		1.452e$+$04 	\minus	&		    1.553e$+$04 	\minus	&		    1.478e$+$04 	\minus	&	\win	8.473e$+$03 	\\
                                &                           &	    	(1.566e$+$03) 		    &	    	(5.006e$+$02) 		    &	 \worst	(4.960e$+$02) 		        &	   	(2.762e$+$03) 		        &		    (2.759e$+$03) 		    &		    (5.178e$+$02) 		    &		(2.680e$+$03) 		        &		(9.413e$+$02) 		    &		    (6.615e$+$02) 		    &		    (7.739e$+$02) 		    &	\win	(1.569e$+$03) 	\\
                                &	\multirow{2}{*}{100}	&	    	3.298e$+$04 	\minus	&	    	3.325e$+$04 	\minus	&	       	3.345e$+$04 	\minus	    &	   	3.277e$+$04 	\minus	    &		    2.960e$+$04 	\minus	&		    3.343e$+$04 	\minus	&		3.359e$+$04 	\minus	    &		3.151e$+$04 	\minus	&	\worst	3.360e$+$04 	\minus	&		    3.292e$+$04 	\minus	&	\win	2.511e$+$04 	\\
                                &                           &	    	(1.443e$+$03) 		    &	    	(6.660e$+$02) 		    &	       	(7.473e$+$02) 		        &	   	(8.774e$+$02) 		        &		    (3.907e$+$03) 		    &		    (8.071e$+$02) 		    &		(5.983e$+$02) 		        &		(1.659e$+$03) 		    &	\worst	(7.457e$+$02) 		    &		    (8.305e$+$02) 		    &	\win	(4.549e$+$03) 	\\ \hline
            \multirow{6}{*}{F3} &	\multirow{2}{*}{30}		&	    	1.712e$+$02 	\minus	&	\worst	1.816e$+$03 	\minus	&	       	2.469e$+$02 	\minus	    &	   	3.406e$+$02 	\minus	    &		    2.163e$+$02 	\minus	&		    1.485e$+$02 	\minus	&		1.307e$+$02 	\minus	    &		5.085e$+$02 	\minus	&		    8.738e$+$02 	\minus	&	\win	1.001e$+$02 	\plus	&		    1.133e$+$02 	\\
                                &                           &	    	(4.296e$+$01) 		    &	\worst	(2.083e$+$02) 		    &	       	(1.767e$+$01) 		        &	   	(4.377e$+$01) 		        &		    (6.779e$+$01) 		    &		    (3.003e$+$01) 		    &		(2.742e$+$01) 		        &		(5.345e$+$01) 		    &		    (2.183e$+$02) 		    &	\win	(2.557e$+$01) 		    &		    (2.052e$+$01) 	\\
                                &	\multirow{2}{*}{50}		&	    	5.046e$+$02 	\minus	&	\worst	3.912e$+$03 	\minus	&	       	4.762e$+$02 	\minus	    &	   	7.111e$+$02 	\minus	    &		    5.109e$+$02 	\minus	&		    4.379e$+$02 	\minus	&		4.736e$+$02 	\minus	    &		1.061e$+$03 	\minus	&		    2.674e$+$03 	\minus	&		    4.585e$+$02 	\minus	&	\win	2.656e$+$02 	\\
                                &                           &	    	(1.281e$+$02) 		    &	\worst	(4.569e$+$02) 		    &	       	(3.093e$+$01) 		        &	   	(1.580e$+$02) 		        &		    (1.260e$+$02) 		    &		    (9.539e$+$01) 		    &		(1.676e$+$01) 		        &		(9.555e$+$01) 		    &		    (1.148e$+$03) 		    &		    (3.509e$+$01) 		    &	\win	(5.934e$+$01) 	\\
                                &	\multirow{2}{*}{100}	&	    	1.683e$+$03 	\minus	&	    	1.100e$+$04 	\minus	&	   \win	1.067e$+$03 	\plus	    &	   	2.145e$+$03 	\minus	    &		    2.118e$+$03 	\minus	&		    2.467e$+$03 	\minus	&		1.525e$+$03 	\minus	    &		2.569e$+$03 	\minus	&	\worst	1.132e$+$04 	\minus	&		    1.130e$+$03 	\plus	&		    1.447e$+$03 	\\
                                &                           &	    	(1.695e$+$02) 		    &	    	(5.319e$+$02) 		    &	   \win	(5.035e$+$01) 		        &	   	(3.241e$+$02) 		        &		    (2.264e$+$02) 		    &		    (2.751e$+$02) 		    &		(6.307e$+$01) 		        &		(1.383e$+$02) 		    &	\worst	(7.086e$+$02) 		    &		    (4.037e$+$01) 		    &		    (1.448e$+$02) 	\\ \hline
            \multirow{6}{*}{F4} &	\multirow{2}{*}{30}		&	    	6.513e$+$06 	\minus	&	    	1.719e$+$06 	\minus	&	       	3.362e$+$01 	\nodiff	    &	   	7.877e$+$03 	\minus	    &		    2.569e$+$01 	\plus	&	\win	2.441e$+$01 	\plus	&		5.717e$+$06 	\minus	    &		5.594e$+$04 	\minus	&	\worst	1.249e$+$07 	\minus	&		    2.978e$+$02 	\minus	&		    3.157e$+$01 	\\
                                &                           &	    	(2.962e$+$06) 		    &	    	(1.321e$+$06) 		    &	       	(1.286e$+$01) 		        &	   	(1.541e$+$04) 		        &		    (4.324e$+$00) 		    &	\win	(7.758e$+$00) 		    &		(1.036e$+$07) 		        &		(7.029e$+$04) 		    &	\worst	(5.799e$+$06) 		    &		    (1.314e$+$02) 		    &		    (7.378e$+$00) 	\\
                                &	\multirow{2}{*}{50}		&	    	4.328e$+$07 	\minus	&	    	2.286e$+$07 	\minus	&	   \win	1.888e$+$02 	\plus	    &	   	3.700e$+$03 	\minus	    &		    6.509e$+$02 	\plus	&		    2.024e$+$02 	\plus	&		1.080e$+$06 	\minus	    &		6.918e$+$05 	\minus	&	\worst	9.473e$+$07 	\minus	&		    2.246e$+$04 	\minus	&		    1.583e$+$03 	\\
                                &                           &	    	(1.568e$+$07) 		    &	    	(1.105e$+$07) 		    &	   \win	(2.143e$+$02) 		        &	   	(1.679e$+$03) 		        &		    (6.771e$+$02) 		    &		    (1.716e$+$02) 		    &		(7.446e$+$05) 		        &		(4.774e$+$05) 		    &	\worst	(4.242e$+$07) 		    &		    (1.364e$+$04) 		    &		    (9.694e$+$02) 	\\
                                &	\multirow{2}{*}{100}	&	    	1.786e$+$08 	\minus	&	    	2.368e$+$08 	\minus	&	   \win	5.821e$+$03 	\plus	    &	   	1.902e$+$06 	\minus	    &		    9.467e$+$05 	\nodiff	&		    7.120e$+$05 	\nodiff	&		1.318e$+$07 	\minus	    &		1.395e$+$07 	\minus	&	\worst	6.151e$+$08 	\minus	&		    7.427e$+$06 	\minus	&		    8.491e$+$05 	\\
                                &                           &	    	(7.931e$+$07) 		    &	    	(1.013e$+$08) 		    &	   \win	(3.901e$+$03) 		        &	   	(6.720e$+$06) 		        &		    (5.533e$+$05) 		    &		    (4.277e$+$05) 		    &		(8.432e$+$06) 		        &		(6.745e$+$06) 		    &	\worst	(2.288e$+$08) 		    &		    (3.291e$+$06) 		    &		    (4.465e$+$05) 	\\ \hline
            \multirow{6}{*}{F5} &	\multirow{2}{*}{30}		&	    	1.825e$+$07 	\minus	&	    	2.076e$+$07 	\minus	&	       	2.070e$+$07 	\minus	    &	   	5.891e$+$07 	\minus	    &		    7.290e$+$06 	\minus	&	\win	1.775e$+$06 	\nodiff	&	\worst	1.448e$+$08 	\minus	&		1.854e$+$07 	\minus	&		    6.796e$+$07 	\minus	&		    1.196e$+$07 	\minus	&		    2.247e$+$06 	\\
                                &                           &	    	(7.039e$+$06) 		    &	    	(1.366e$+$07) 		    &	       	(1.109e$+$07) 		        &	   	(2.902e$+$07) 		        &		    (5.219e$+$06) 		    &	\win	(1.026e$+$06) 		    &	\worst	(6.443e$+$07) 		    &		(1.069e$+$07) 		    &		    (4.028e$+$07) 		    &		    (6.235e$+$06) 		    &		    (1.632e$+$06) 	\\
                                &	\multirow{2}{*}{50}		&	    	8.245e$+$07 	\minus	&	    	2.318e$+$08 	\minus	&	       	6.062e$+$07 	\minus	    &	   	1.355e$+$08 	\minus	    &		    2.806e$+$07 	\minus	&	\win	6.179e$+$06 	\plus	&		1.266e$+$08 	\minus	    &		1.135e$+$08 	\minus	&	\worst	3.895e$+$08 	\minus	&		    5.877e$+$07 	\minus	&		    9.154e$+$06 	\\
                                &                           &	    	(3.841e$+$07) 		    &	    	(9.925e$+$07) 		    &	       	(2.630e$+$07) 		        &	   	(1.356e$+$08) 		        &		    (1.865e$+$07) 		    &	\win	(5.059e$+$06) 		    &		(1.481e$+$08) 		        &		(5.925e$+$07) 		    &	\worst	(1.721e$+$08) 		    &		    (2.845e$+$07) 		    &		    (5.061e$+$06) 	\\
                                &	\multirow{2}{*}{100}	&	    	1.499e$+$08 	\minus	&	    	1.288e$+$09 	\minus	&	       	2.805e$+$08 	\minus	    &	   	3.123e$+$08 	\minus	    &		    1.221e$+$08 	\minus	&	\win	9.129e$+$07 	\nodiff	&		5.340e$+$08 	\minus	    &		3.094e$+$08 	\minus	&	\worst	1.723e$+$09 	\minus	&		    2.721e$+$08 	\minus	&		    1.023e$+$08 	\\
                                &                           &	    	(8.444e$+$07) 		    &	    	(3.217e$+$08) 		    &	       	(1.106e$+$08) 		        &	   	(3.244e$+$08) 		        &		    (5.295e$+$07) 		    &	\win	(4.401e$+$07) 		    &		(3.998e$+$08) 		        &		(8.142e$+$07) 		    &	\worst	(4.980e$+$08) 		    &		    (6.886e$+$07) 		    &		    (4.225e$+$07) 	\\ \hline
            \multirow{6}{*}{F6} &	\multirow{2}{*}{30}		&	    	2.921e$+$03 	\minus	&	    	2.620e$+$03 	\minus	&	       	2.008e$+$03 	\minus	    &	   	1.859e$+$03 	\minus	    &		    1.072e$+$03 	\nodiff	&	\win	1.006e$+$03 	\nodiff	&		2.654e$+$03 	\minus	    &		2.258e$+$03 	\minus	&	\worst	3.311e$+$03 	\minus	&		    1.112e$+$03 	\nodiff	&		    1.081e$+$03 	\\
                                &                           &	    	(2.752e$+$02) 		    &	    	(3.403e$+$02) 		    &	       	(2.797e$+$02) 		        &	   	(5.843e$+$02) 		        &		    (3.331e$+$02) 		    &	\win	(3.789e$+$02) 		    &		(1.499e$+$03) 		        &		(3.973e$+$02) 		    &	\worst	(3.182e$+$02) 		    &		    (3.166e$+$02) 		    &		    (3.104e$+$02) 	\\
                                &	\multirow{2}{*}{50}		&	    	6.361e$+$03 	\minus	&	    	6.746e$+$03 	\minus	&	       	4.401e$+$03 	\minus	    &	   	4.626e$+$03 	\minus	    &		    2.617e$+$03 	\minus	&	\win	2.088e$+$03 	\nodiff	&		4.101e$+$03 	\minus	    &		4.704e$+$03 	\minus	&	\worst	8.422e$+$03 	\minus	&		    3.381e$+$03 	\minus	&		    2.183e$+$03 	\\
                                &                           &	    	(5.535e$+$02) 		    &	    	(1.079e$+$03) 		    &	       	(4.155e$+$02) 		        &	   	(6.365e$+$02) 		        &		    (6.368e$+$02) 		    &	\win	(4.678e$+$02) 		    &		(6.273e$+$02) 		        &		(5.569e$+$02) 		    &	\worst	(8.649e$+$02) 		    &		    (4.875e$+$02) 		    &		    (4.928e$+$02) 	\\
                                &	\multirow{2}{*}{100}	&	    	1.210e$+$04 	\minus	&	\worst	2.758e$+$04 	\minus	&	       	1.000e$+$04 	\minus	    &	   	1.202e$+$04 	\minus	    &		    7.160e$+$03 	\nodiff	&		    7.743e$+$03 	\minus	&		1.149e$+$04 	\minus	    &		1.265e$+$04 	\minus	&		    2.610e$+$04 	\minus	&		    1.013e$+$04 	\minus	&	\win	7.133e$+$03 	\\
                                &                           &	    	(9.428e$+$02) 		    &	\worst	(4.540e$+$03) 		    &	       	(6.941e$+$02) 		        &	   	(2.019e$+$03) 		        &		    (9.212e$+$02) 		    &		    (7.100e$+$02) 		    &		(7.483e$+$02) 		        &		(9.496e$+$02) 		    &		    (3.192e$+$03) 		    &		    (5.205e$+$02) 		    &	\win	(9.144e$+$02) 	\\ \hline
            \multirow{6}{*}{F7} &	\multirow{2}{*}{30}		&	    	9.296e$+$06 	\minus	&	    	4.921e$+$06 	\minus	&	       	7.286e$+$06 	\minus	    &	   	2.359e$+$07 	\minus	    &		    2.192e$+$06 	\minus	&	\win	4.991e$+$05 	\nodiff	&	\worst	8.214e$+$07 	\minus	&		1.110e$+$07 	\minus	&		    4.489e$+$07 	\minus	&		    6.061e$+$06 	\minus	&		    5.363e$+$05 	\\
                                &                           &	    	(5.326e$+$06) 		    &	    	(5.090e$+$06) 		    &	       	(4.090e$+$06) 		        &	   	(8.314e$+$06) 		        &		    (1.728e$+$06) 		    &	\win	(6.649e$+$05) 		    &	\worst	(4.049e$+$07) 		    &		(8.252e$+$06) 		    &		    (2.171e$+$07) 		    &		    (3.344e$+$06) 		    &		    (5.347e$+$05) 	\\
                                &	\multirow{2}{*}{50}		&	    	5.880e$+$07 	\minus	&	    	4.117e$+$07 	\minus	&	       	2.670e$+$07 	\minus	    &	   	3.484e$+$07 	\minus	    &		    1.768e$+$07 	\minus	&	\win	4.201e$+$06 	\nodiff	&		5.091e$+$07 	\minus	    &		2.564e$+$07 	\minus	&	\worst	1.500e$+$08 	\minus	&		    1.663e$+$07 	\minus	&		    5.235e$+$06 	\\
                                &                           &	    	(2.252e$+$07) 		    &	    	(1.549e$+$07) 		    &	       	(1.193e$+$07) 		        &	   	(1.986e$+$07) 		        &		    (1.112e$+$07) 		    &	\win	(2.773e$+$06) 		    &		(6.817e$+$07) 		        &		(1.417e$+$07) 		    &	\worst	(6.233e$+$07) 		    &		    (7.553e$+$06) 		    &		    (4.438e$+$06) 	\\
                                &	\multirow{2}{*}{100}	&	    	1.413e$+$08 	\minus	&	    	5.609e$+$08 	\minus	&	       	1.849e$+$08 	\minus	    &	   	2.134e$+$08 	\minus	    &		    6.268e$+$07 	\minus	&	\win	3.225e$+$07 	\plus	&		3.026e$+$08 	\minus	    &		1.314e$+$08 	\minus	&	\worst	8.029e$+$08 	\minus	&		    1.575e$+$08 	\minus	&		    4.524e$+$07 	\\
                                &                           &	    	(5.231e$+$07) 		    &	    	(2.077e$+$08) 		    &	       	(7.307e$+$07) 		        &	   	(6.797e$+$07) 		        &		    (2.957e$+$07) 		    &	\win	(1.430e$+$07) 		    &		(1.359e$+$08) 		        &		(4.524e$+$07) 		    &	\worst	(2.452e$+$08) 		    &		    (3.535e$+$07) 		    &		    (1.529e$+$07) 	\\ \hline
            \multirow{6}{*}{F8} &	\multirow{2}{*}{30}		&	    	4.993e$+$03 	\minus	&	    	8.421e$+$03 	\minus	&	       	3.089e$+$03 	\nodiff	    &	   	3.830e$+$03 	\nodiff	    &		    5.392e$+$03 	\minus	&		    3.844e$+$03 	\nodiff	&		7.076e$+$03 	\minus	    &		3.667e$+$03 	\nodiff	&	\worst	8.461e$+$03 	\minus	&	\win	1.246e$+$02 	\plus	&		    3.095e$+$03 	\\
                                &                           &	    	(2.399e$+$03) 		    &	    	(8.060e$+$02) 		    &	       	(4.060e$+$03) 		        &	   	(1.929e$+$03) 		        &		    (3.269e$+$03) 		    &		    (3.795e$+$03) 		    &		(1.518e$+$03) 		        &		(3.244e$+$03) 		    &	\worst	(9.433e$+$02) 		    &	\win	(4.648e$+$01) 		    &		    (2.470e$+$03) 	\\
                                &	\multirow{2}{*}{50}		&	    	1.518e$+$04 	\minus	&	\worst	1.578e$+$04 	\minus	&	       	1.546e$+$04 	\minus	    &	   	1.374e$+$04 	\minus	    &		    1.176e$+$04 	\minus	&		    1.534e$+$04 	\minus	&		1.461e$+$04 	\minus	    &		1.372e$+$04 	\minus	&		    1.575e$+$04 	\minus	&		    1.122e$+$04 	\minus	&	\win	8.854e$+$03 	\\
                                &                           &	    	(1.489e$+$03) 		    &	\worst	(5.454e$+$02) 		    &	       	(1.344e$+$03) 		        &	   	(2.095e$+$03) 		        &		    (3.523e$+$03) 		    &		    (2.002e$+$03) 		    &		(1.509e$+$03) 		        &		(2.371e$+$03) 		    &		    (6.461e$+$02) 		    &		    (5.668e$+$03) 		    &	\win	(1.607e$+$03) 	\\
                                &	\multirow{2}{*}{100}	&	    	3.403e$+$04 	\minus	&	    	3.447e$+$04 	\minus	&	 \worst	3.467e$+$04 	\minus	    &	   	3.366e$+$04 	\minus	    &		    2.878e$+$04 	\minus	&		    3.423e$+$04 	\minus	&		3.370e$+$04 	\minus	    &		3.300e$+$04 	\minus	&		    3.460e$+$04 	\minus	&		    3.334e$+$04 	\minus	&	\win	2.511e$+$04 	\\
                                &                           &	    	(9.781e$+$02) 		    &	    	(8.517e$+$02) 		    &	 \worst	(6.117e$+$02) 		        &	   	(6.402e$+$02) 		        &		    (4.090e$+$03) 		    &		    (1.980e$+$03) 		    &		(7.985e$+$02) 		        &		(1.805e$+$03) 		    &		    (8.150e$+$02) 		    &		    (6.052e$+$02) 		    &	\win	(3.821e$+$03) 	\\ \hline
            \multirow{6}{*}{F9} &	\multirow{2}{*}{30}		&	    	5.829e$+$02 	\minus	&	\worst	8.752e$+$02 	\minus	&	       	6.797e$+$02 	\minus	    &	   	6.360e$+$02 	\minus	    &		    5.318e$+$02 	\minus	&	\win	4.708e$+$02 	\plus	&		5.810e$+$02 	\minus	    &		7.515e$+$02 	\minus	&		    7.704e$+$02 	\minus	&		    4.846e$+$02 	\nodiff	&		    4.927e$+$02 	\\
                                &                           &	    	(2.854e$+$01) 		    &	\worst	(7.384e$+$01) 		    &	       	(3.074e$+$01) 		        &	   	(7.443e$+$01) 		        &		    (3.000e$+$01) 		    &	\win	(1.260e$+$01) 		    &		(5.823e$+$01) 		        &		(5.246e$+$01) 		    &		    (4.021e$+$01) 		    &		    (1.677e$+$01) 		    &		    (2.211e$+$01) 	\\
                                &	\multirow{2}{*}{50}		&	    	8.150e$+$02 	\minus	&	\worst	1.507e$+$03 	\minus	&	       	9.816e$+$02 	\minus	    &	   	9.625e$+$02 	\minus	    &		    7.340e$+$02 	\minus	&	\win	6.562e$+$02 	\nodiff	&		9.361e$+$02 	\minus	    &		1.278e$+$03 	\minus	&		    1.297e$+$03 	\minus	&		    9.173e$+$02 	\minus	&		    6.831e$+$02 	\\
                                &                           &	    	(5.406e$+$01) 		    &	\worst	(2.338e$+$02) 		    &	       	(4.140e$+$01) 		        &	   	(1.422e$+$02) 		        &		    (5.317e$+$01) 		    &	\win	(5.035e$+$01) 		    &		(3.164e$+$01) 		        &		(1.133e$+$02) 		    &		    (6.443e$+$01) 		    &		    (4.484e$+$01) 		    &		    (7.685e$+$01) 	\\
                                &	\multirow{2}{*}{100}	&	\win	1.939e$+$03 	\plus	&	\worst	4.694e$+$03 	\minus	&	       	2.042e$+$03 	\nodiff	    &	   	2.747e$+$03 	\minus	    &		    2.049e$+$03 	\nodiff	&		    3.452e$+$03 	\minus	&		2.029e$+$03 	\plus	    &		3.061e$+$03 	\minus	&		    3.822e$+$03 	\minus	&		    2.067e$+$03 	\nodiff	&		    2.121e$+$03 	\\
                                &                           &	\win	(1.440e$+$02) 		    &	\worst	(7.766e$+$02) 		    &	       	(5.693e$+$01) 		        &	   	(4.534e$+$02) 		        &		    (1.586e$+$02) 		    &		    (3.533e$+$02) 		    &		(3.363e$+$01) 		        &		(2.219e$+$02) 		    &		    (2.201e$+$02) 		    &		    (5.305e$+$01) 		    &		    (1.708e$+$02) 	\\ \hline
            \multirow{6}{*}{F10}&	\multirow{2}{*}{30}		&	    	7.924e$+$02 	\minus	&	\worst	4.383e$+$03 	\minus	&	       	4.418e$+$02 	\minus	    &	   	4.718e$+$02 	\minus	    &	\win	4.051e$+$02 	\plus	&		    4.190e$+$02 	\nodiff	&		8.503e$+$02 	\minus	    &		1.130e$+$03 	\minus	&		    3.943e$+$03 	\minus	&		    4.426e$+$02 	\minus	&		    4.214e$+$02 	\\
                                &                           &	    	(2.027e$+$02) 		    &	\worst	(1.257e$+$03) 		    &	       	(2.006e$+$01) 		        &	   	(1.099e$+$02) 		        &	\win	(1.987e$+$01) 		    &		    (1.992e$+$01) 		    &		(1.807e$+$02) 		        &		(2.293e$+$02) 		    &		    (1.453e$+$03) 		    &		    (1.251e$+$01) 		    &		    (1.557e$+$01) 	\\
                                &	\multirow{2}{*}{50}		&	    	1.159e$+$03 	\minus	&	\worst	2.687e$+$04 	\minus	&	       	7.197e$+$02 	\minus	    &	   	1.017e$+$03 	\minus	    &	\win	6.497e$+$02 	\plus	&		    7.363e$+$02 	\minus	&		2.129e$+$03 	\minus	    &		4.888e$+$03 	\minus	&		    1.682e$+$04 	\minus	&		    7.434e$+$02 	\minus	&		    6.830e$+$02 	\\
                                &                           &	    	(2.083e$+$02) 		    &	\worst	(3.827e$+$03) 		    &	       	(7.451e$+$01) 		        &	   	(9.231e$+$02) 		        &	\win	(4.465e$+$01) 		    &		    (6.070e$+$01) 		    &		(2.713e$+$02) 		        &		(9.591e$+$02) 		    &		    (5.542e$+$03) 		    &		    (2.967e$+$01) 		    &		    (3.482e$+$01) 	\\
                                &	\multirow{2}{*}{100}	&	    	2.803e$+$03 	\plus	&	    	7.996e$+$04 	\minus	&	   \win	1.505e$+$03 	\plus	    &	   	4.806e$+$03 	\nodiff	    &		    2.755e$+$03 	\plus	&		    7.006e$+$03 	\minus	&		7.764e$+$03 	\minus	    &		1.310e$+$04 	\minus	&	\worst	8.624e$+$04 	\minus	&		    5.134e$+$03 	\minus	&		    3.004e$+$03 	\\
                                &                           &	    	(3.423e$+$02) 		    &	    	(1.275e$+$04) 		    &	   \win	(1.383e$+$02) 		        &	   	(3.931e$+$03) 		        &		    (3.062e$+$02) 		    &		    (1.349e$+$03) 		    &		(7.139e$+$02) 		        &		(1.766e$+$03) 		    &	\worst	(2.251e$+$04) 		    &		    (5.055e$+$02) 		    &		    (3.472e$+$02) 	\\ \hline
            \multicolumn{2}{c|}{$+/-/\sim$}	                &	    	2/28/0		            &	    	0/30/0		            &	   	7/20/3		                    &	   	0/27/3		                &		5/20/5		                &		5/15/10		                &		1/29/0		                &		0/29/1		            &		0/30/0		                &		4/23/3		                &	    	-	            \\
            \multicolumn{2}{c|}{Ave. Rank}	                &	       	6.567 		            &	       	9.700 		            &	   	5.133 		                    &	   	6.233 		                &	   	3.600 	   	                &	   	3.933 	   	                &	   	6.900 	   	                &	   	7.200 	   	            &	   \worst	10.467 	   	        &	   	3.967 	   	                &	   \win	2.300    	    \\ \hline
        \end{tabular}
    }
\end{table*}

\begin{figure*}[t]
    \begin{minipage}[t]{\textwidth}
        \centering
        \begin{minipage}[t]{0.195\textwidth} \centering \includegraphics[width = \textwidth]{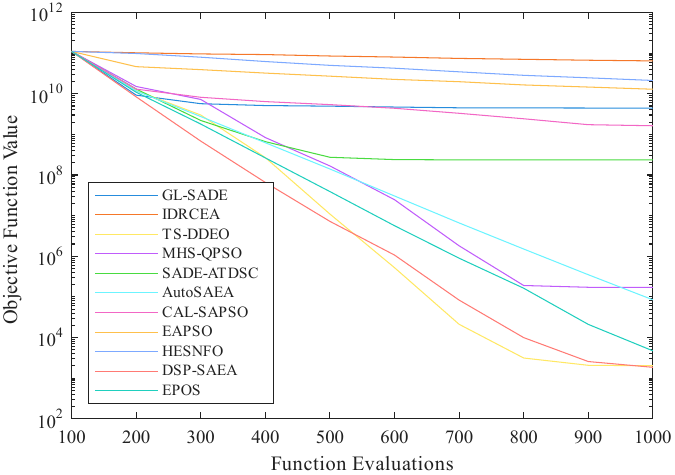} \\ F1 \end{minipage}
        \begin{minipage}[t]{0.195\textwidth} \centering \includegraphics[width = \textwidth]{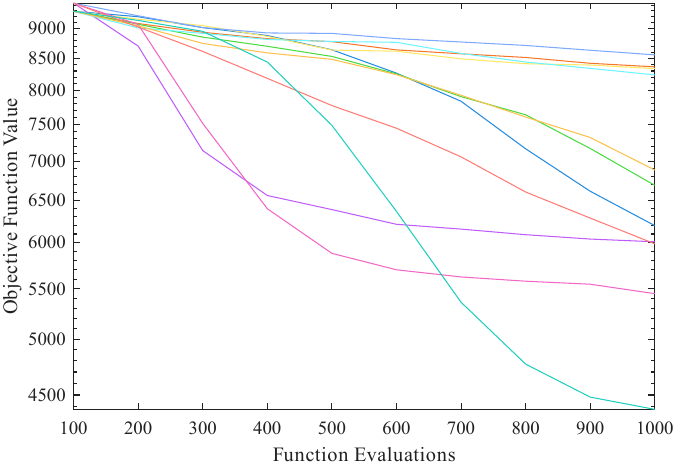} \\ F2 \end{minipage}
        \begin{minipage}[t]{0.195\textwidth} \centering \includegraphics[width = \textwidth]{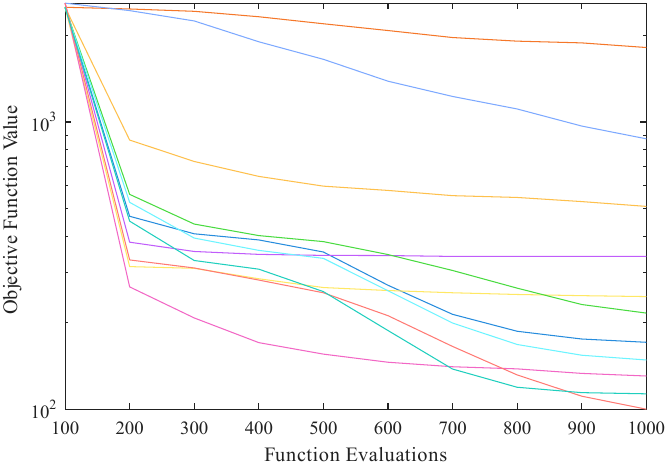} \\ F3 \end{minipage}
        \begin{minipage}[t]{0.195\textwidth} \centering \includegraphics[width = \textwidth]{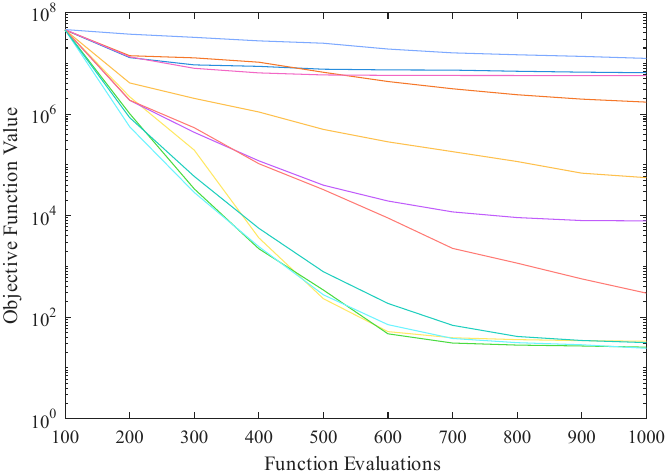} \\ F4 \end{minipage}
        \begin{minipage}[t]{0.195\textwidth} \centering \includegraphics[width = \textwidth]{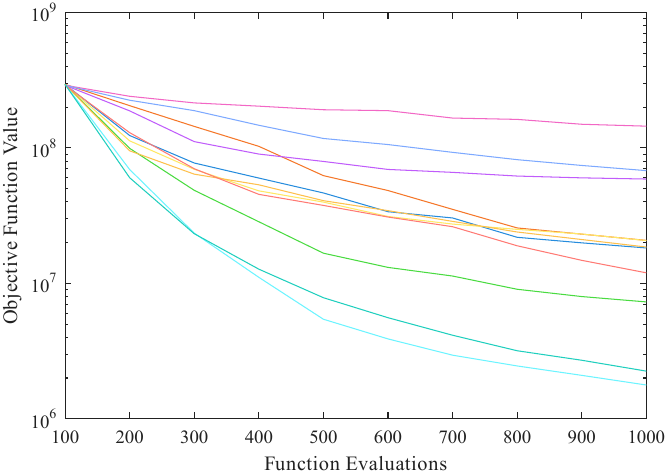} \\ F5 \end{minipage}
        \\\vspace{4mm}
        \begin{minipage}[t]{0.195\textwidth} \centering \includegraphics[width = \textwidth]{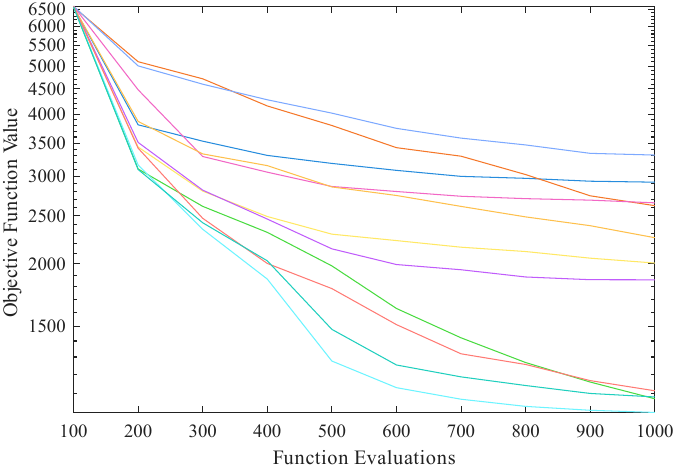} \\ F6 \end{minipage}
        \begin{minipage}[t]{0.195\textwidth} \centering \includegraphics[width = \textwidth]{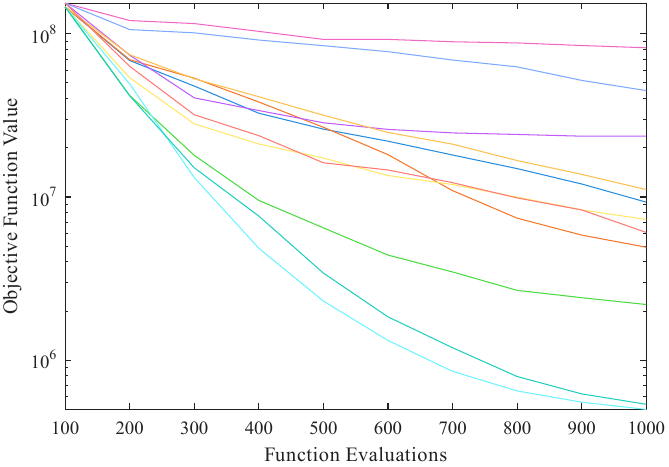} \\ F7 \end{minipage}
        \begin{minipage}[t]{0.195\textwidth} \centering \includegraphics[width = \textwidth]{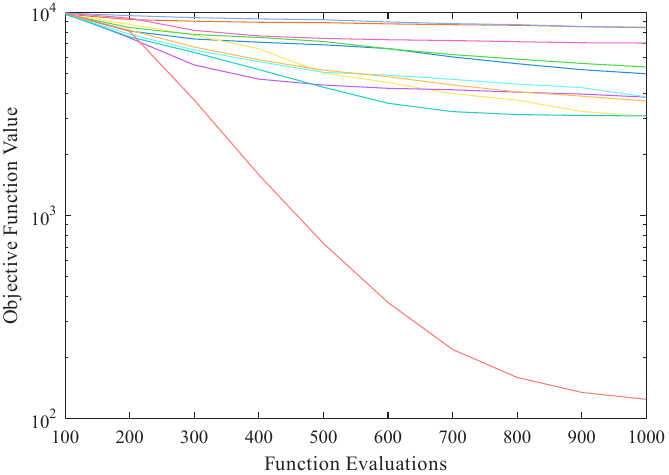} \\ F8 \end{minipage}
        \begin{minipage}[t]{0.195\textwidth} \centering \includegraphics[width = \textwidth]{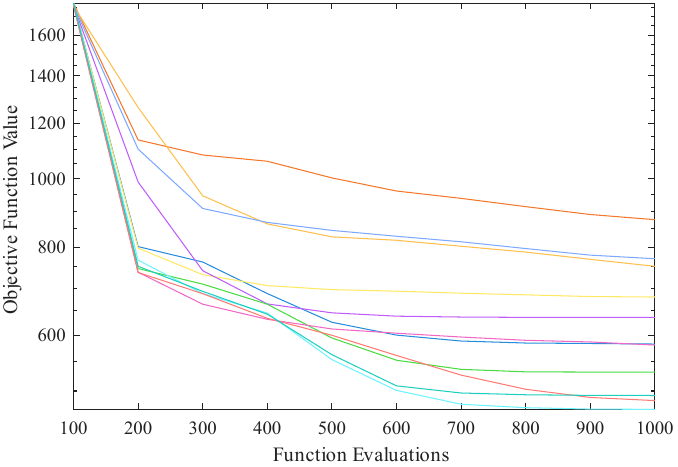} \\ F9 \end{minipage}
        \begin{minipage}[t]{0.195\textwidth} \centering \includegraphics[width = \textwidth]{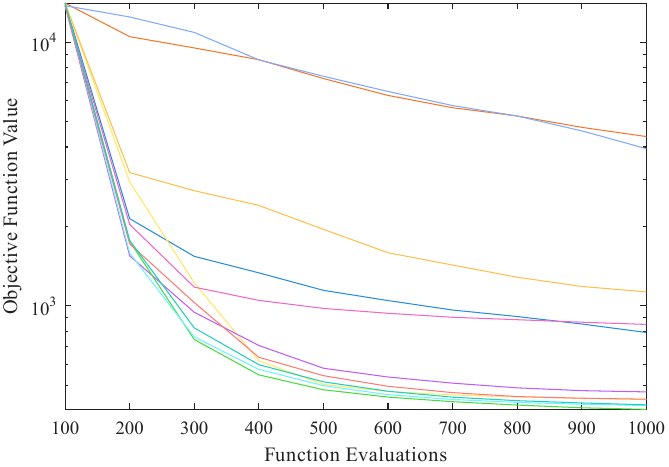} \\ F10 \end{minipage}
        \\\vspace{3mm}
        a) $D=30$
    \end{minipage}
    \\\vspace{5mm}\\
    \begin{minipage}[t]{\textwidth}
        \centering
        \begin{minipage}[t]{0.195\textwidth} \centering \includegraphics[width = \textwidth]{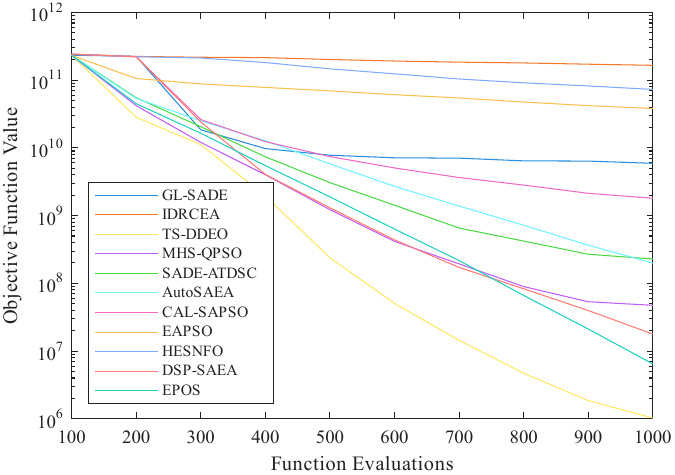} \\ F1 \end{minipage}
        \begin{minipage}[t]{0.195\textwidth} \centering \includegraphics[width = \textwidth]{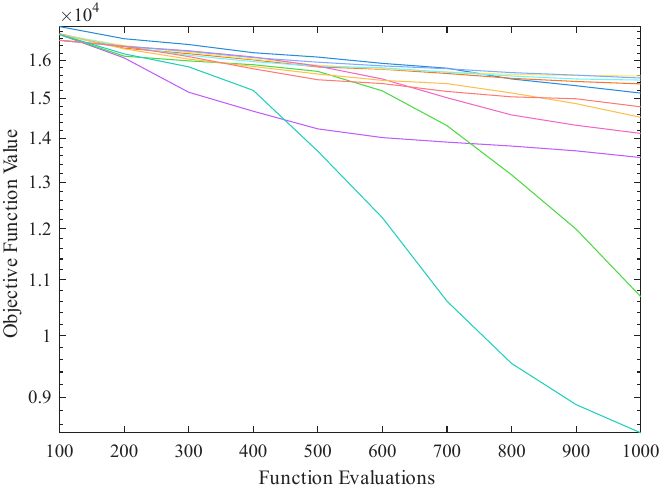} \\ F2 \end{minipage}
        \begin{minipage}[t]{0.195\textwidth} \centering \includegraphics[width = \textwidth]{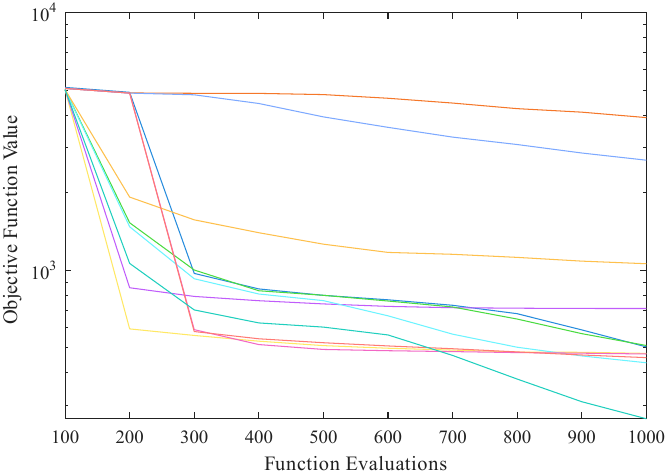} \\ F3 \end{minipage}
        \begin{minipage}[t]{0.195\textwidth} \centering \includegraphics[width = \textwidth]{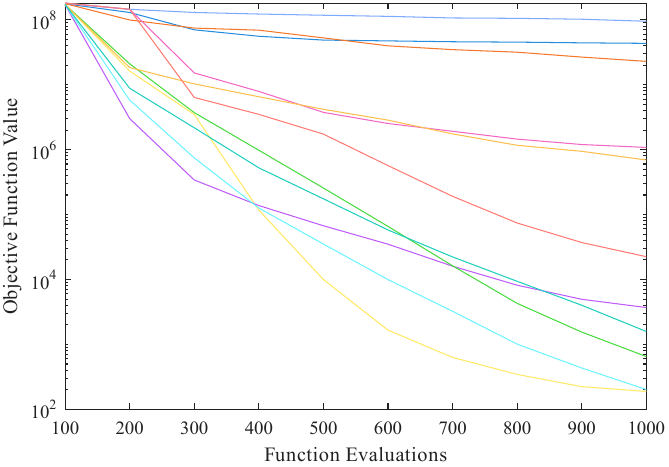} \\ F4 \end{minipage}
        \begin{minipage}[t]{0.195\textwidth} \centering \includegraphics[width = \textwidth]{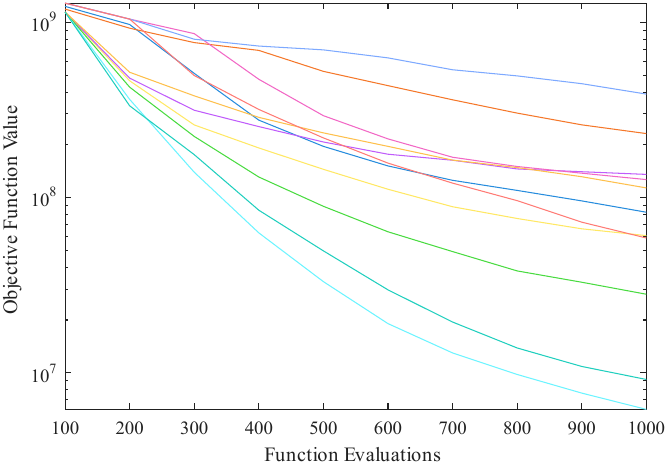} \\ F5 \end{minipage}
        \\\vspace{4mm}
        \begin{minipage}[t]{0.195\textwidth} \centering \includegraphics[width = \textwidth]{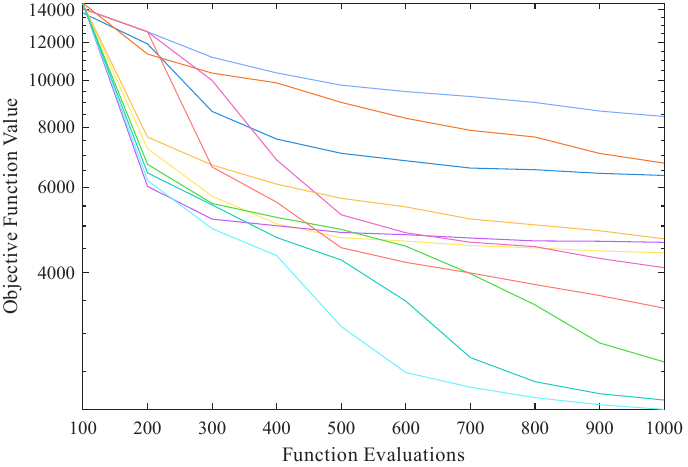} \\ F6 \end{minipage}
        \begin{minipage}[t]{0.195\textwidth} \centering \includegraphics[width = \textwidth]{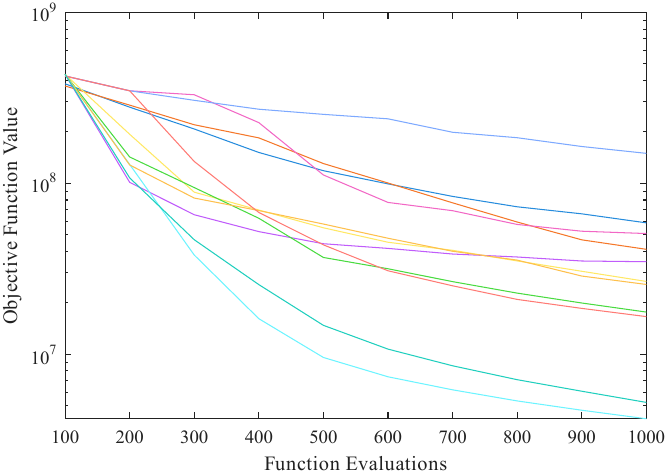} \\ F7 \end{minipage}
        \begin{minipage}[t]{0.195\textwidth} \centering \includegraphics[width = \textwidth]{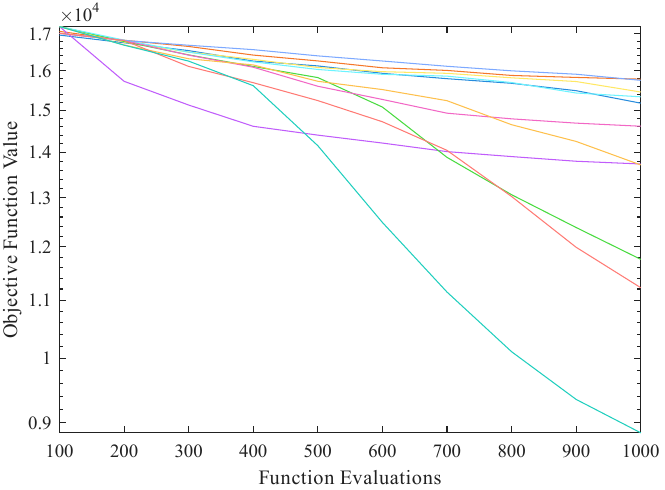} \\ F8 \end{minipage}
        \begin{minipage}[t]{0.195\textwidth} \centering \includegraphics[width = \textwidth]{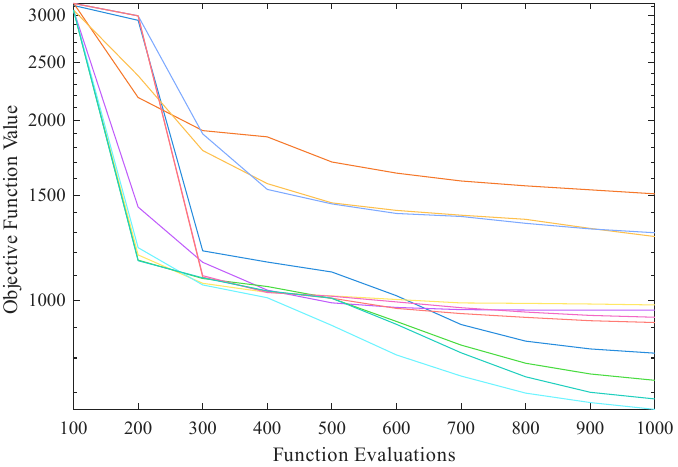} \\ F9 \end{minipage}
        \begin{minipage}[t]{0.195\textwidth} \centering \includegraphics[width = \textwidth]{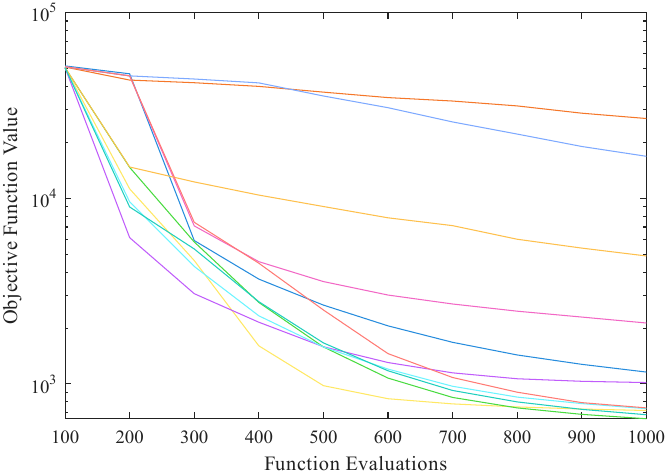} \\ F10 \end{minipage}
        \\\vspace{3mm}
        b) $D=50$
    \end{minipage}
    \\\vspace{5mm}\\
    \begin{minipage}[t]{\textwidth}
        \centering
        \begin{minipage}[t]{0.195\textwidth} \centering \includegraphics[width = \textwidth]{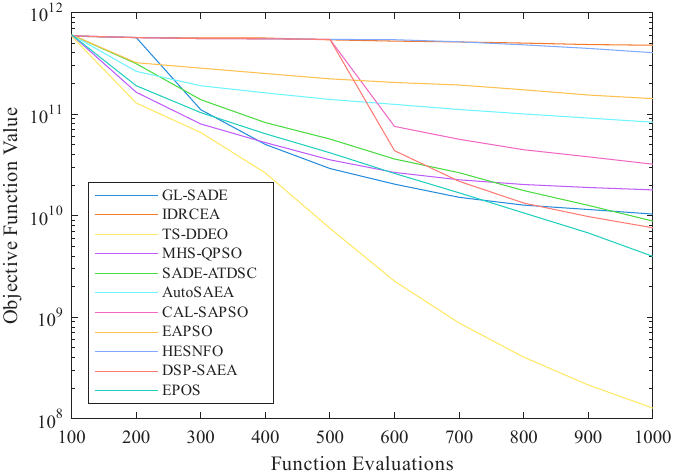} \\ F1 \end{minipage}
        \begin{minipage}[t]{0.195\textwidth} \centering \includegraphics[width = \textwidth]{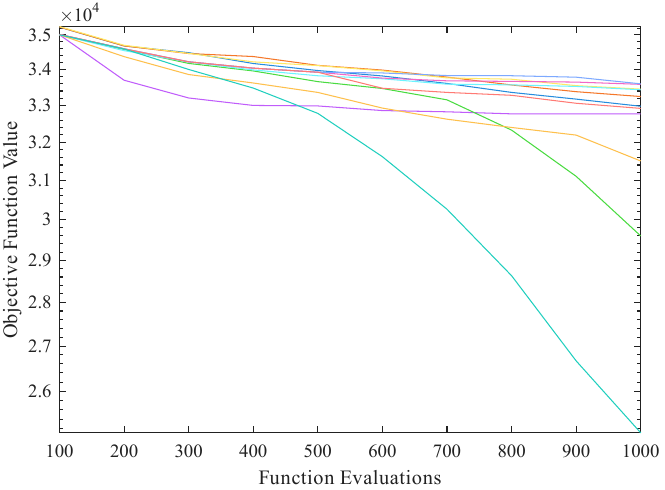} \\ F2 \end{minipage}
        \begin{minipage}[t]{0.195\textwidth} \centering \includegraphics[width = \textwidth]{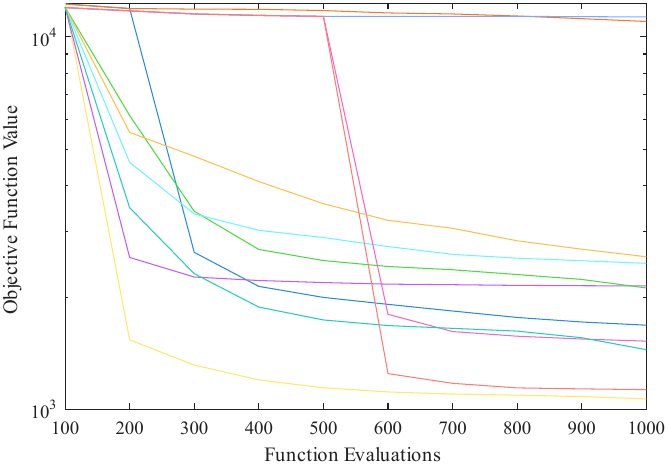} \\ F3 \end{minipage}
        \begin{minipage}[t]{0.195\textwidth} \centering \includegraphics[width = \textwidth]{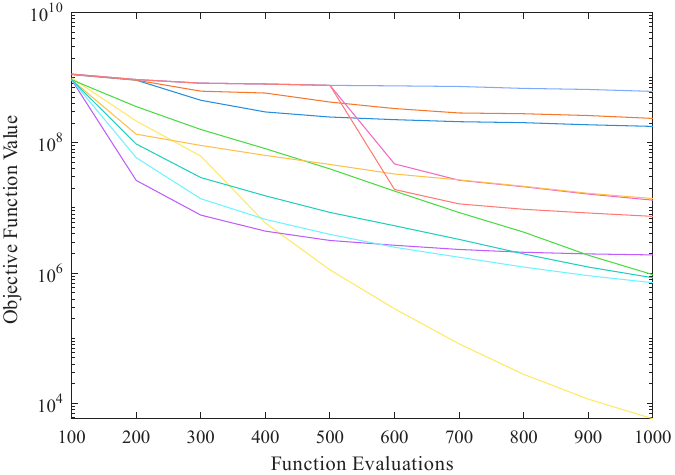} \\ F4 \end{minipage}
        \begin{minipage}[t]{0.195\textwidth} \centering \includegraphics[width = \textwidth]{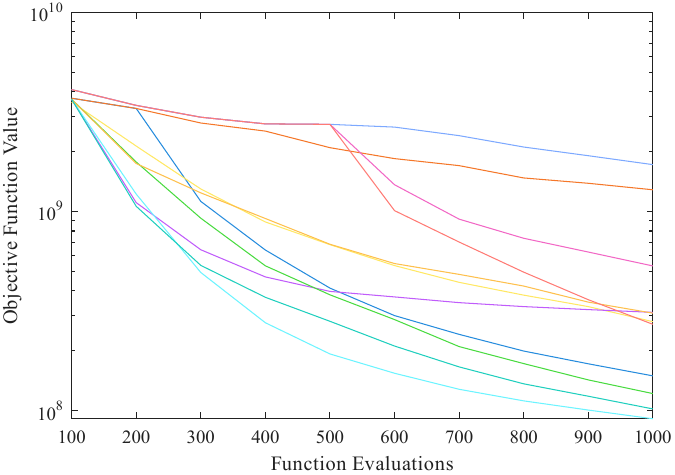} \\ F5 \end{minipage}
        \\\vspace{4mm}
        \begin{minipage}[t]{0.195\textwidth} \centering \includegraphics[width = \textwidth]{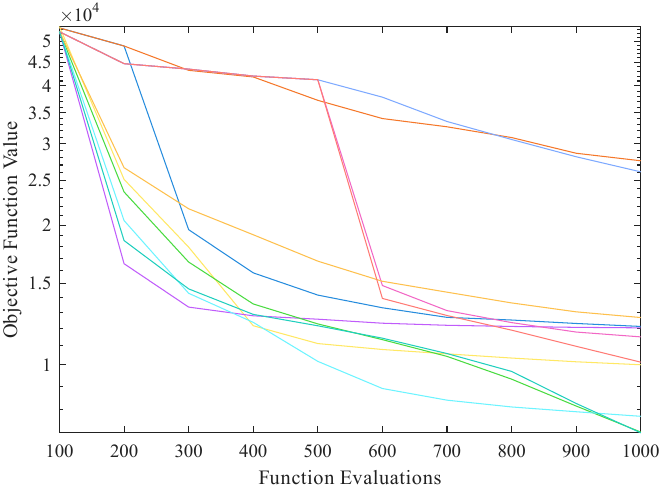} \\ F6 \end{minipage}
        \begin{minipage}[t]{0.195\textwidth} \centering \includegraphics[width = \textwidth]{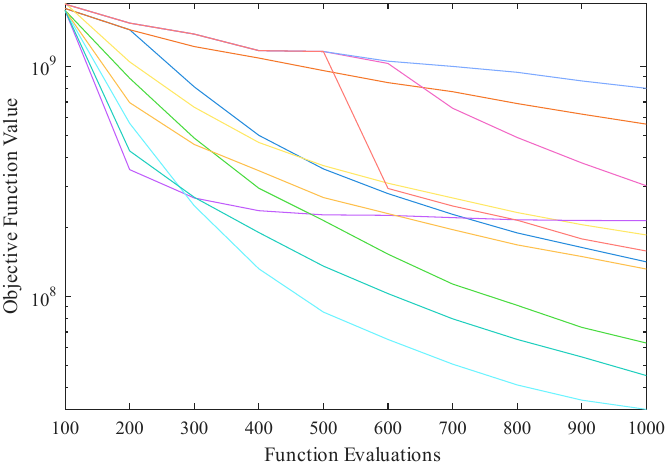} \\ F7 \end{minipage}
        \begin{minipage}[t]{0.195\textwidth} \centering \includegraphics[width = \textwidth]{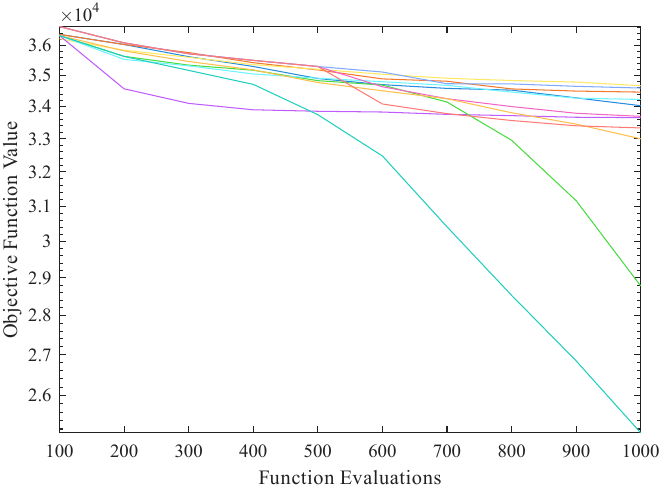} \\ F8 \end{minipage}
        \begin{minipage}[t]{0.195\textwidth} \centering \includegraphics[width = \textwidth]{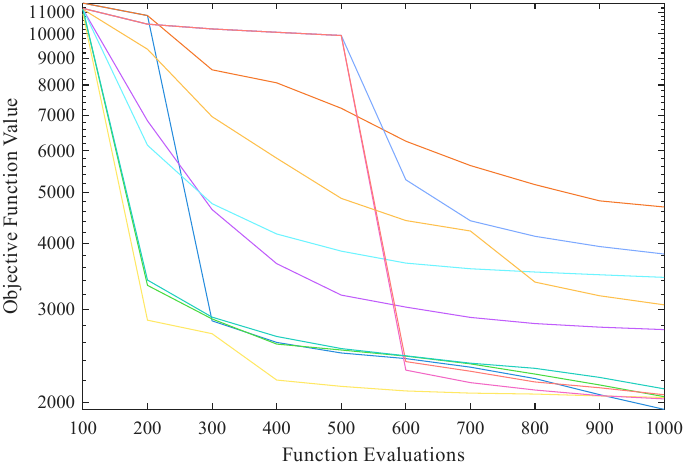} \\ F9 \end{minipage}
        \begin{minipage}[t]{0.195\textwidth} \centering \includegraphics[width = \textwidth]{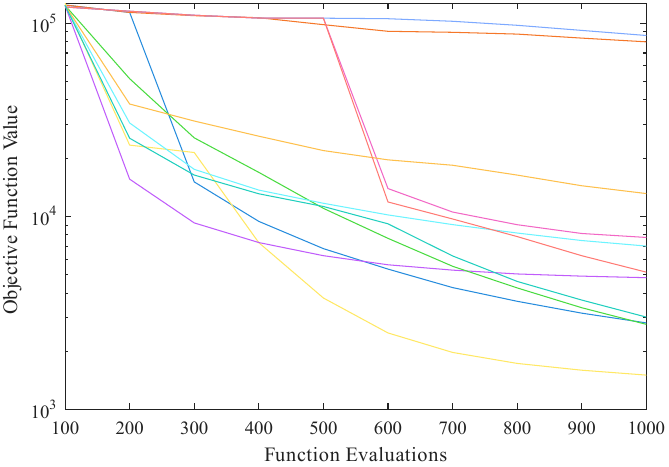} \\ F10 \end{minipage}
        \\\vspace{3mm}
        c) $D=100$
    \end{minipage}
    \caption{The convergence curves obtained in the experiments on the CEC2020 Benchmark Problem Suite in Section~\ref{sec:exp}.}
    \label{fig:convergence_curve}
\end{figure*}

\begin{table*}[t]
    \renewcommand{\arraystretch}{1.4}
    \centering
    \caption{The average fitness values discovered at $1,000$ fitness evaluations on the CEC2011 Real-world Problem Suite.}
    % \vspace{1mm}
    \label{tab:appx-data_CEC2011RW}
    \begin{minipage}[t]{\textwidth}
        \centering
        \scalebox{0.75}{
            \begin{tabular}{l|r|cccc|cc|cc|ccc}\hline\hline
                                        &							& \multicolumn{4}{c|}{Normal SAEAs}                                                                                                                     & \multicolumn{2}{c|}{Adaptive SAEAs}                           & \multicolumn{2}{c|}{Ensemble SAEAs}                           & \multicolumn{3}{c}{Adaptive Ensemble SAEAs}                                           \\
                ID                      &	\multicolumn{1}{c|}{$D$}& GL-SADE                           & IDRCEA                        & TS-DDEO                                   & MHS-QPSO                            & SADE-ATDSC                    & AutoSAEA                      & CAL-SAPSO                     & EAPSO                         & HESNFO                        & DSP-SAEA                      & \ours                 \\\hline
                \multirow{2}{*}{F1}	    & \multirow{2}{*}{6}     	&		2.466e$+$01 	\minus	    &		2.698e$+$01 	\minus	&			2.588e$+$01 	\minus		&			2.364e$+$01 	\nodiff		&	\win	2.163e$+$01 	\nodiff	&		2.196e$+$01 	\nodiff	&		2.761e$+$01 	\minus	&		2.316e$+$01 	\nodiff	&	\worst	2.814e$+$01 	\minus	&		2.358e$+$01 	\nodiff	&		2.266e$+$01 \\
                                        &                           &		(2.074e$+$00) 		        &		(1.155e$+$00) 		&			(1.294e$+$00) 			&			(4.361e$+$00) 		&	\win	(7.190e$+$00) 		&		(3.076e$+$00) 		&		(1.356e$+$00) 		&		(3.227e$+$00) 		&	\worst	(8.305e$-$01) 		&		(2.931e$+$00) 		&		(3.046e$+$00) \\
                \multirow{2}{*}{F2}	    & \multirow{2}{*}{30}    	&		-2.598e$+$00 	\minus	    &		-3.969e$+$00 	\minus	&			-6.933e$+$00 	\minus		&			-6.457e$+$00 	\minus		&		-4.778e$+$00 	\minus	&		-9.103e$+$00 	\nodiff	&		-2.582e$+$00 	\minus	&		-4.732e$+$00 	\minus	&	\worst	-2.303e$+$00 	\minus	&	\win	-1.006e$+$01 	\nodiff	&		-9.655e$+$00 \\
                                        &                           &		(5.298e$-$01) 		        &		(1.254e$+$00) 		&			(1.849e$+$00) 			&			(9.245e$-$01) 			&		(1.797e$+$00) 		&		(1.850e$+$00) 		&		(4.413e$-$01) 		&		(9.718e$-$01) 		&	\worst	(4.004e$-$01) 		&	\win	(2.678e$+$00) 		&		(3.093e$+$00) \\
                \multirow{2}{*}{F3}	    & \multirow{2}{*}{1}     	&		1.152e$-$05 	\minus	    &		1.152e$-$05 	\nodiff	&			1.152e$-$05 	\nodiff		&			1.152e$-$05 	\minus		&	\win	1.152e$-$05 	\plus	&		1.152e$-$05 	\plus	&		1.152e$-$05 	\minus	&		1.152e$-$05 	\nodiff	&	\worst	1.174e$-$05 	\minus	&		1.152e$-$05 	\minus	&		1.152e$-$05 \\
                                        &                           &		(1.018e$-$12) 		        &		(4.672e$-$19) 		&			(6.018e$-$19) 			&			(2.730e$-$14) 			&	\win	(4.247e$-$19) 		&		(3.717e$-$19) 		&		(8.939e$-$09) 		&		(5.531e$-$19) 		&	\worst	(4.558e$-$07) 		&		(2.766e$-$13) 		&		(1.289e$-$18) \\
                \multirow{2}{*}{F4}	    & \multirow{2}{*}{1}     	&		2.186e$+$01 	\minus	    &		1.928e$+$01 	\plus	&			2.007e$+$01 	\nodiff		&		\win	1.881e$+$01 	\plus		&		2.102e$+$01 	\minus	&		2.115e$+$01 	\minus	&	\worst	2.950e$+$01 	\minus	&		2.164e$+$01 	\minus	&		2.255e$+$01 	\minus	&		1.921e$+$01 	\nodiff	&		2.043e$+$01 \\
                                        &                           &		(6.926e$-$01) 		        &		(2.878e$+$00) 		&			(2.244e$+$00) 			&		\win	(2.820e$+$00) 			&		(1.830e$+$00) 		&		(1.415e$+$00) 		&	\worst	(4.671e$+$00) 		&		(5.052e$-$01) 		&		(9.550e$-$01) 		&		(2.966e$+$00) 		&		(2.209e$+$00) \\
                \multirow{2}{*}{F5}	    & \multirow{2}{*}{30}    	&	\worst	-9.918e$+$00 	\minus	&		-1.424e$+$01 	\minus	&			-1.410e$+$01 	\minus		&			-1.714e$+$01 	\minus		&		-1.491e$+$01 	\minus	&	\win	-2.420e$+$01 	\nodiff	&		-1.243e$+$01 	\minus	&		-1.740e$+$01 	\minus	&		-1.037e$+$01 	\minus	&		-1.263e$+$01 	\minus	&		-2.262e$+$01 \\
                                        &                           &	\worst	(1.896e$+$00) 		    &		(2.264e$+$00) 		&			(1.669e$+$00) 			&			(3.765e$+$00) 			&		(2.470e$+$00) 		&	\win	(4.765e$+$00) 		&		(2.190e$+$00) 		&		(2.357e$+$00) 		&		(1.716e$+$00) 		&		(2.688e$+$00) 		&		(4.554e$+$00) \\
                \multirow{2}{*}{F6}	    & \multirow{2}{*}{30}    	&	\worst	N/A	\minus	            &		-5.133e$-$01 	\minus	&			-8.750e$+$00 	\nodiff		&			-5.867e$+$00 	\nodiff		&		-7.915e$+$00 	\nodiff	&	\win	-1.816e$+$01 	\plus	&		9.988e$+$00 	\minus	&		-9.691e$+$00 	\nodiff	&		6.220e$+$01 	\minus	&		2.769e$+$00 	\minus	&		-5.195e$+$00 \\
                                        &                           &	\worst	(N/A)		            &		(8.079e$+$00) 		&			(2.094e$+$00) 			&			(4.281e$+$00) 			&		(3.410e$+$00) 		&	\win	(3.442e$+$00) 		&		(2.752e$+$01) 		&		(1.831e$+$00) 		&		(1.099e$+$02) 		&		(1.210e$+$01) 		&		(2.145e$+$01) \\
                \multirow{2}{*}{F7}	    & \multirow{2}{*}{20}    	&		1.623e$+$00 	\nodiff	    &		2.419e$+$00 	\minus	&			2.439e$+$00 	\minus		&			2.027e$+$00 	\minus		&	\win	1.421e$+$00 	\plus	&		1.685e$+$00 	\nodiff	&	\worst	2.504e$+$00 	\minus	&		1.950e$+$00 	\minus	&		2.192e$+$00 	\minus	&		1.817e$+$00 	\minus	&		1.600e$+$00 \\
                                        &                           &		(2.725e$-$01) 		        &		(1.875e$-$01) 		&			(1.872e$-$01) 			&			(3.496e$-$01) 			&	\win	(3.031e$-$01) 		&		(4.180e$-$01) 		&	\worst	(3.509e$-$01) 		&		(2.620e$-$01) 		&		(3.322e$-$01) 		&		(2.337e$-$01) 		&		(2.511e$-$01) \\
                \multirow{2}{*}{F8}	    & \multirow{2}{*}{7}     	&		5.469e$+$02 	\minus	    &		3.036e$+$02 	\nodiff	&			3.135e$+$02 	\nodiff		&			3.448e$+$02 	\nodiff		&	\win	2.759e$+$02 	\nodiff	&		3.075e$+$02 	\nodiff	&	\worst	9.431e$+$02 	\minus	&		2.932e$+$02 	\nodiff	&		8.381e$+$02 	\minus	&		5.919e$+$02 	\minus	&		3.071e$+$02 \\
                                        &                           &		(4.001e$+$02) 		        &		(1.405e$+$02) 		&			(1.395e$+$02) 			&			(2.355e$+$02) 			&	\win	(4.663e$+$01) 		&		(1.121e$+$02) 		&	\worst	(7.268e$+$02) 		&		(8.951e$+$01) 		&		(6.933e$+$02) 		&		(4.487e$+$02) 		&		(8.201e$+$01) \\
                \multirow{2}{*}{F9}	    & \multirow{2}{*}{126}   	&		9.608e$+$04 	\plus	    &		1.948e$+$05 	\plus	&			1.204e$+$05 	\plus		&			5.308e$+$05 	\minus		&	\win	7.949e$+$04 	\plus	&	\worst	1.214e$+$06 	\minus	&		5.346e$+$05 	\minus	&		4.937e$+$05 	\minus	&		9.885e$+$05 	\minus	&		6.372e$+$05 	\minus	&		2.872e$+$05 \\
                                        &                           &		(6.682e$+$04) 		&		(8.173e$+$04) 		&			(5.437e$+$04) 			&			(2.026e$+$05) 			&	\win	(4.656e$+$04) 		&	\worst	(1.331e$+$05) 		&		(7.140e$+$04) 		&		(2.045e$+$05) 		&		(2.920e$+$05) 		&		(4.586e$+$04) 		&		(1.248e$+$05) \\
                \multirow{2}{*}{F10}	& \multirow{2}{*}{12}    	&		-9.625e$+$00 	\minus	&	\worst	-7.135e$+$00 	\minus	&			-7.698e$+$00 	\minus		&			-8.243e$+$00 	\minus		&		-1.319e$+$01 	\nodiff	&	\win	-1.523e$+$01 	\plus	&		-1.035e$+$01 	\minus	&		-1.049e$+$01 	\minus	&		-9.340e$+$00 	\minus	&		-1.032e$+$01 	\minus	&		-1.299e$+$01 \\
                                        &                           &		(8.183e$-$01) 		&	\worst	(1.080e$+$00) 		&			(9.311e$-$01) 			&			(1.218e$+$00) 			&		(2.776e$+$00) 		&	\win	(2.471e$+$00) 		&		(4.141e$-$01) 		&		(1.805e$+$00) 		&		(7.588e$-$01) 		&		(3.227e$-$01) 		&		(2.342e$+$00) \\
                \multirow{2}{*}{F11-1}	& \multirow{2}{*}{120}   	&		2.551e$+$06 	\minus	&		1.159e$+$08 	\minus	&		\win	1.411e$+$06 	\plus		&			1.841e$+$06 	\plus		&		2.343e$+$06 	\minus	&		2.308e$+$06 	\minus	&		6.753e$+$06 	\minus	&		2.273e$+$06 	\minus	&	\worst	2.704e$+$08 	\minus	&		5.597e$+$06 	\minus	&		2.104e$+$06 \\
                                        &                           &		(3.331e$+$05) 		&		(6.805e$+$07) 		&		\win	(2.497e$+$05) 			&			(2.597e$+$05) 			&		(3.512e$+$05) 		&		(2.188e$+$05) 		&		(2.050e$+$06) 		&		(3.360e$+$05) 		&	\worst	(3.746e$+$07) 		&		(4.438e$+$05) 		&		(1.994e$+$05) \\
                \multirow{2}{*}{F11-2}	& \multirow{2}{*}{216}   	&		2.248e$+$06 	\plus	&		5.310e$+$06 	\minus	&		\win	2.158e$+$06 	\plus		&			6.646e$+$06 	\minus		&		2.880e$+$06 	\nodiff	&		6.322e$+$06 	\minus	&	\worst	1.399e$+$07 	\minus	&		5.834e$+$06 	\minus	&	\worst	1.399e$+$07 	\minus	&	\worst	1.399e$+$07 	\minus	&		2.913e$+$06 \\
                                        &                           &		(2.133e$+$05) 		&		(3.613e$+$05) 		&		\win	(3.113e$+$05) 			&			(5.147e$+$05) 			&		(3.296e$+$05) 		&		(4.025e$+$05) 		&	\worst	(5.375e$+$05) 		&		(3.389e$+$05) 		&	\worst	(5.375e$+$05) 		&	\worst	(5.375e$+$05) 		&		(3.138e$+$05) \\
                \multirow{2}{*}{F11-3}	& \multirow{2}{*}{6}     	&		1.554e$+$04 	\nodiff	&		3.071e$+$04 	\minus	&			1.605e$+$04 	\minus		&		\worst	5.784e$+$04 	\minus		&		1.554e$+$04 	\nodiff	&	\win	1.548e$+$04 	\plus	&		3.313e$+$04 	\minus	&		1.572e$+$04 	\minus	&		1.905e$+$04 	\minus	&		2.016e$+$04 	\nodiff	&		1.553e$+$04 \\
                                        &                           &		(4.895e$+$01) 		&		(1.847e$+$04) 		&			(8.815e$+$02) 			&		\worst	(4.885e$+$04) 			&		(4.799e$+$01) 		&	\win	(2.109e$+$01) 		&		(3.133e$+$04) 		&		(1.702e$+$02) 		&		(1.450e$+$04) 		&		(1.361e$+$04) 		&		(5.239e$+$01) \\
                \multirow{2}{*}{F11-4}	& \multirow{2}{*}{13}    	&		1.935e$+$04 	\nodiff	&	\worst	7.546e$+$04 	\minus	&			5.647e$+$04 	\minus		&			2.135e$+$04 	\minus		&		2.630e$+$04 	\minus	&		1.939e$+$04 	\nodiff	&		3.115e$+$04 	\minus	&		2.325e$+$04 	\minus	&		2.697e$+$04 	\minus	&		2.672e$+$04 	\minus	&	\win	1.933e$+$04 \\
                                        &                           &		(2.147e$+$02) 		&	\worst	(7.995e$+$04) 		&			(5.415e$+$04) 			&			(2.294e$+$03) 			&		(5.272e$+$03) 		&		(2.081e$+$02) 		&		(1.460e$+$04) 		&		(3.293e$+$03) 		&		(8.750e$+$03) 		&		(1.653e$+$04) 		&	\win	(1.951e$+$02) \\
                \multirow{2}{*}{F11-5}	& \multirow{2}{*}{15}    	&		3.346e$+$04 	\plus	&		1.280e$+$06 	\minus	&			3.361e$+$04 	\plus		&			3.945e$+$05 	\minus		&	\win	3.317e$+$04 	\nodiff	&		3.319e$+$04 	\nodiff	&		2.618e$+$05 	\minus	&		6.644e$+$04 	\minus	&		3.075e$+$05 	\minus	&	\worst	4.268e$+$06 	\minus	&		3.521e$+$04 \\
                                        &                           &		(7.629e$+$02) 		&		(1.012e$+$06) 		&			(7.856e$+$02) 			&			(9.517e$+$04) 			&	\win	(1.264e$+$02) 		&		(8.354e$+$01) 		&		(1.275e$+$05) 		&		(4.915e$+$04) 		&		(5.044e$+$05) 		&	\worst	(3.321e$+$06) 		&		(1.145e$+$04) \\
                \multirow{2}{*}{F11-6}	& \multirow{2}{*}{40}    	&		1.500e$+$05 	\nodiff	&		2.351e$+$07 	\minus	&			2.207e$+$05 	\minus		&			4.255e$+$05 	\minus		&		1.691e$+$05 	\minus	&	\win	1.441e$+$05 	\nodiff	&		1.587e$+$05 	\minus	&		1.577e$+$05 	\minus	&		1.582e$+$05 	\minus	&	\worst	5.863e$+$07 	\minus	&		1.463e$+$05 \\
                                        &                           &		(8.834e$+$03) 		&		(2.227e$+$07) 		&			(7.066e$+$04) 			&			(1.103e$+$06) 			&		(2.041e$+$04) 		&	\win	(4.840e$+$03) 		&		(8.628e$+$03) 		&		(1.092e$+$04) 		&		(1.436e$+$04) 		&	\worst	(1.758e$+$07) 		&		(7.352e$+$03) \\
                \multirow{2}{*}{F11-7}	& \multirow{2}{*}{140}   	&		5.529e$+$08 	\minus	&		1.284e$+$10 	\minus	&			1.468e$+$08 	\minus		&			2.873e$+$09 	\minus		&		1.410e$+$08 	\nodiff	&		1.086e$+$09 	\minus	&		5.321e$+$08 	\minus	&		1.348e$+$09 	\minus	&		7.750e$+$09 	\minus	&	\worst	1.442e$+$10 	\minus	&	\win	1.260e$+$08 \\
                                        &                           &		(8.073e$+$08) 		&		(4.283e$+$09) 		&			(1.838e$+$08) 			&			(7.969e$+$08) 			&		(3.072e$+$08) 		&		(8.793e$+$08) 		&		(3.750e$+$08) 		&		(9.957e$+$08) 		&		(2.068e$+$09) 		&	\worst	(1.694e$+$09) 		&	\win	(3.979e$+$08) \\
                \multirow{2}{*}{F11-8}	& \multirow{2}{*}{96}    	&	\win	1.368e$+$06 	\plus	&		5.207e$+$07 	\minus	&			1.588e$+$07 	\minus		&			3.518e$+$07 	\minus		&		1.535e$+$06 	\nodiff	&		2.193e$+$07 	\minus	&		1.006e$+$07 	\minus	&		1.152e$+$07 	\minus	&	\worst	5.360e$+$07 	\minus	&		4.435e$+$07 	\minus	&		1.515e$+$06 \\
                                        &                           &	\win	(6.933e$+$05) 		&		(3.075e$+$07) 		&			(5.989e$+$06) 			&			(1.421e$+$07) 			&		(6.254e$+$05) 		&		(5.917e$+$06) 		&		(2.973e$+$06) 		&		(8.150e$+$06) 		&	\worst	(2.045e$+$07) 		&		(5.043e$+$06) 		&		(3.951e$+$05) \\
                \multirow{2}{*}{F11-9}	& \multirow{2}{*}{96}    	&	\win	1.618e$+$06 	\plus	&		5.124e$+$07 	\minus	&			1.634e$+$07 	\minus		&			3.080e$+$07 	\minus		&		1.723e$+$06 	\plus	&		2.506e$+$07 	\minus	&		1.024e$+$07 	\minus	&		1.127e$+$07 	\minus	&	\worst	5.394e$+$07 	\minus	&		4.354e$+$07 	\minus	&		2.062e$+$06 \\
                                        &                           &	\win	(5.859e$+$05) 		&		(2.638e$+$07) 		&			(5.601e$+$06) 			&			(6.704e$+$06) 			&		(5.519e$+$05) 		&		(8.152e$+$06) 		&		(5.280e$+$06) 		&		(7.986e$+$06) 		&	\worst	(1.671e$+$07) 		&		(3.374e$+$06) 		&		(6.025e$+$05) \\
                \multirow{2}{*}{F11-10}	& \multirow{2}{*}{96}    	&	\win	1.368e$+$06 	\plus	&		5.207e$+$07 	\minus	&			1.588e$+$07 	\minus		&			3.518e$+$07 	\minus		&		1.535e$+$06 	\nodiff	&		2.193e$+$07 	\minus	&		1.006e$+$07 	\minus	&		1.152e$+$07 	\minus	&	\worst	5.360e$+$07 	\minus	&		4.435e$+$07 	\minus	&		1.515e$+$06 \\
                                        &                           &	\win	(6.933e$+$05) 		&		(3.075e$+$07) 		&			(5.989e$+$06) 			&			(1.421e$+$07) 			&		(6.254e$+$05) 		&		(5.917e$+$06) 		&		(2.973e$+$06) 		&		(8.150e$+$06) 		&	\worst	(2.045e$+$07) 		&		(5.043e$+$06) 		&		(3.951e$+$05) \\
                \multirow{2}{*}{F12}	& \multirow{2}{*}{26}    	&		8.395e$+$01 	\minus	&		5.597e$+$01 	\minus	&			5.767e$+$01 	\minus		&			5.954e$+$01 	\minus		&		4.731e$+$01 	\minus	&		3.466e$+$01 	\nodiff	&		8.415e$+$01 	\minus	&		4.517e$+$01 	\minus	&		7.994e$+$01 	\minus	&	\worst	9.044e$+$01 	\minus	&	\win	3.217e$+$01 \\
                                        &                           &		(1.410e$+$01) 		&		(7.723e$+$00) 		&			(7.510e$+$00) 			&			(6.519e$+$00) 			&		(1.295e$+$01) 		&		(8.708e$+$00) 		&		(1.531e$+$01) 		&		(9.306e$+$00) 		&		(1.392e$+$01) 		&	\worst	(1.581e$+$01) 		&	\win	(7.704e$+$00) \\
                \multirow{2}{*}{F13}	& \multirow{2}{*}{22}    	&		5.777e$+$01 	\minus	&		5.137e$+$01 	\minus	&			4.962e$+$01 	\minus		&			5.233e$+$01 	\minus		&		3.934e$+$01 	\minus	&	\win	3.212e$+$01 	\nodiff	&		6.580e$+$01 	\minus	&		4.029e$+$01 	\minus	&		6.666e$+$01 	\minus	&	\worst	7.906e$+$01 	\minus	&		3.327e$+$01 \\
                                        &                           &		(9.385e$+$00) 		&		(7.563e$+$00) 		&			(6.396e$+$00) 			&			(5.616e$+$00) 			&		(9.218e$+$00) 		&	\win	(5.892e$+$00) 		&		(9.807e$+$00) 		&		(5.642e$+$00) 		&		(7.908e$+$00) 		&	\worst	(1.103e$+$01) 		&		(8.817e$+$00) \\ \hline
                \multicolumn{2}{c|}{$+/-/\sim$}		                &		6/12/4		&		2/18/2		&			4/14/4			&			2/17/3			&		4/8/10		&		4/8/10		&		0/22/0		&		0/18/4		&		0/22/0		&		0/18/4		&		-\\ 
                \multicolumn{2}{c|}{Ave. Rank}		                &		5.500 		&		7.727 		&			5.591 			&			6.682 			&		3.273 		&		3.909 		&		8.182 		&		4.727 		&	\worst	9.455 		&		8.000 		&	\win	2.955\\ \hline
            \end{tabular}
        }
    \end{minipage}
\end{table*}

\begin{figure*}[t]
    \centering
    \begin{minipage}[t]{0.195\textwidth} \centering \includegraphics[width = \textwidth]{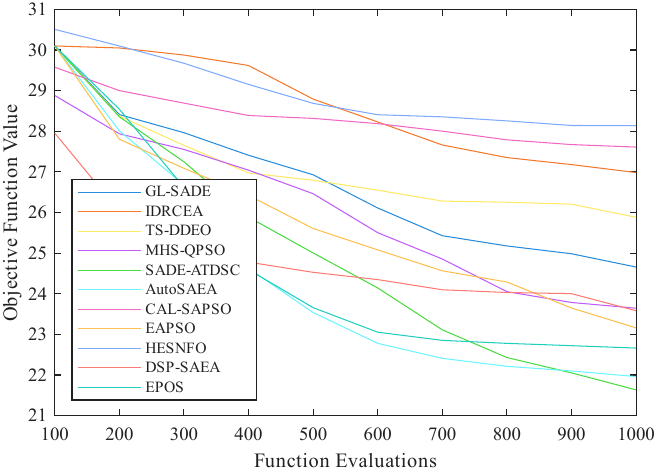} \\ F1 \end{minipage}
    \begin{minipage}[t]{0.195\textwidth} \centering \includegraphics[width = \textwidth]{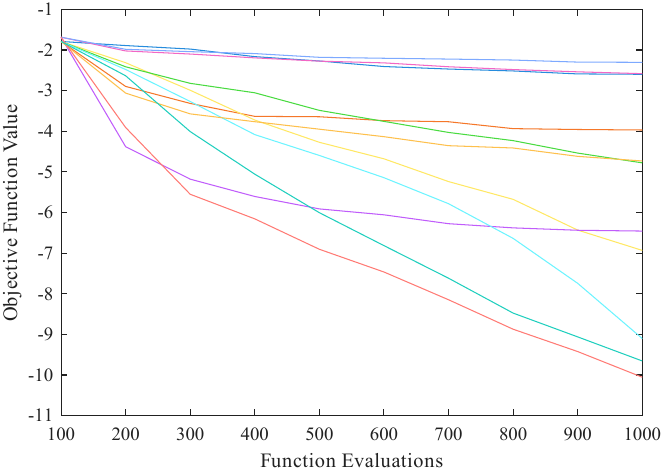} \\ F2 \end{minipage}
    \begin{minipage}[t]{0.195\textwidth} \centering \includegraphics[width = \textwidth]{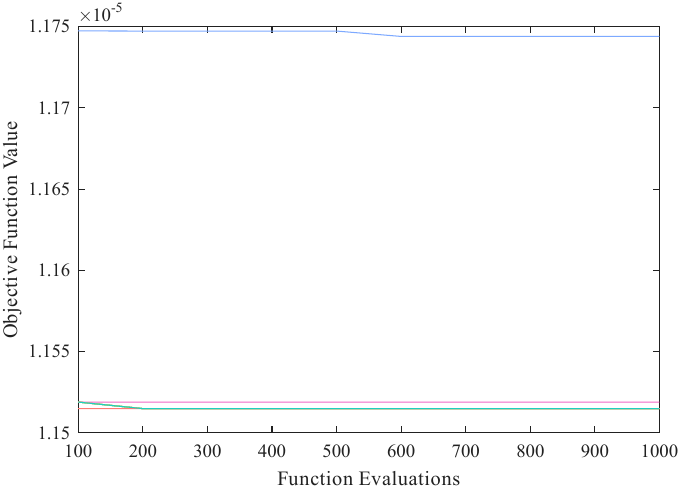} \\ F3 \end{minipage}
    \begin{minipage}[t]{0.195\textwidth} \centering \includegraphics[width = \textwidth]{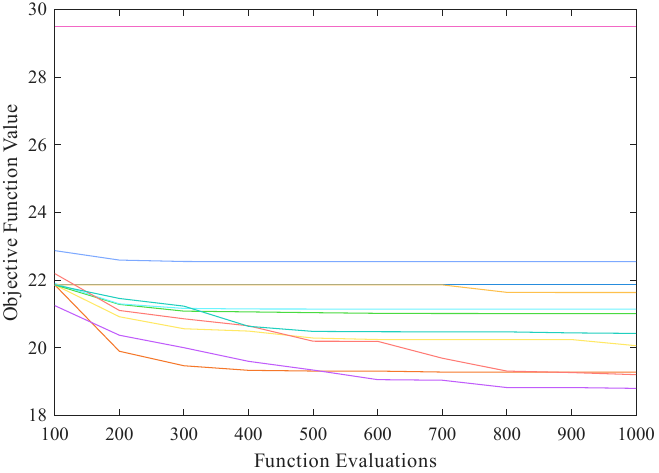} \\ F4 \end{minipage}
    \begin{minipage}[t]{0.195\textwidth} \centering \includegraphics[width = \textwidth]{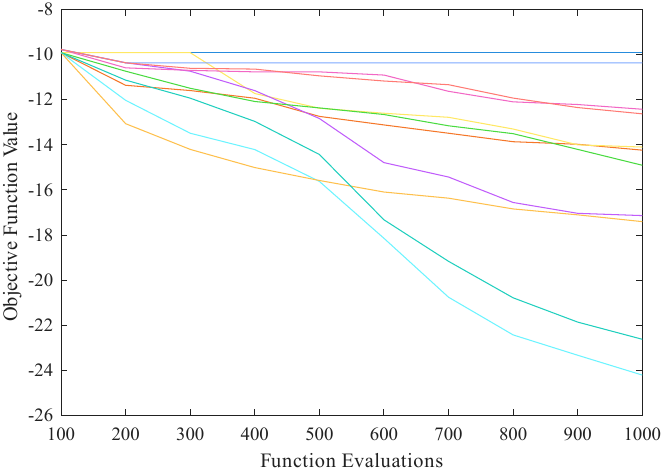} \\ F5 \end{minipage}
    \\\vspace{4mm}
    \begin{minipage}[t]{0.195\textwidth} \centering \includegraphics[width = \textwidth]{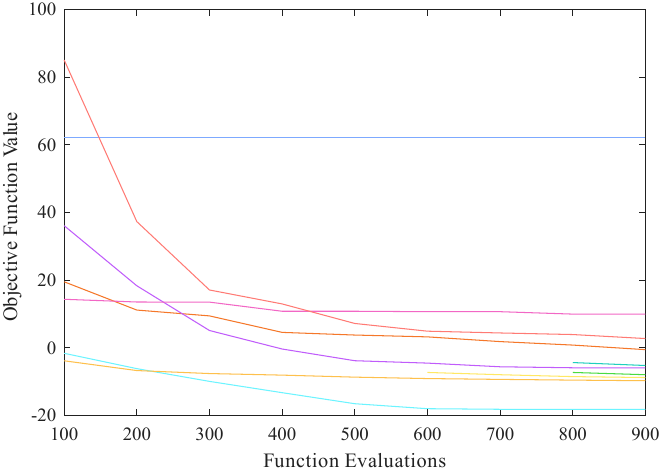} \\ F6 \end{minipage}
    \begin{minipage}[t]{0.195\textwidth} \centering \includegraphics[width = \textwidth]{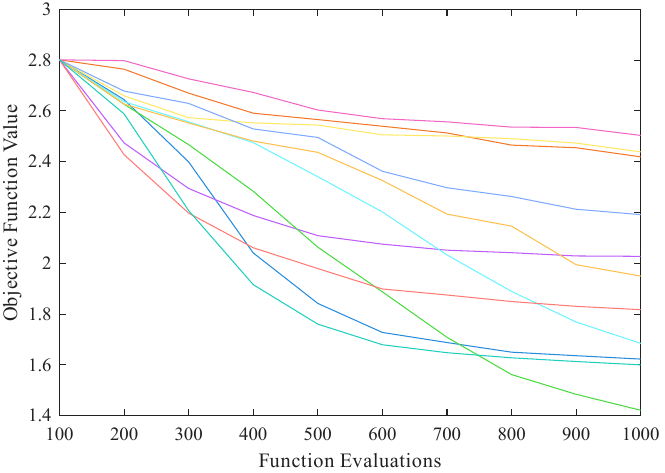} \\ F7 \end{minipage}
    \begin{minipage}[t]{0.195\textwidth} \centering \includegraphics[width = \textwidth]{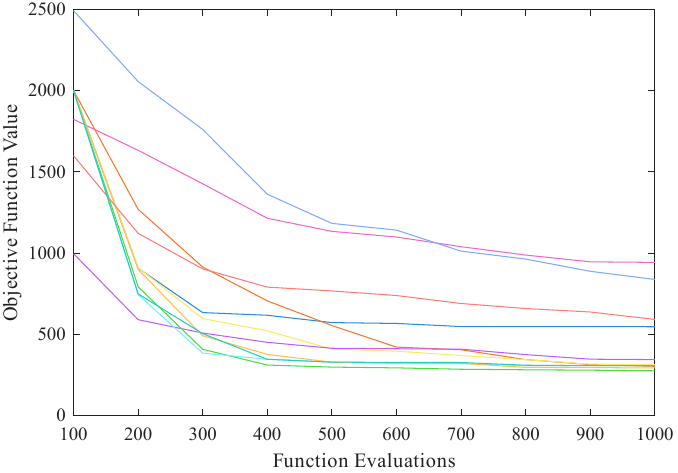} \\ F8 \end{minipage}
    \begin{minipage}[t]{0.195\textwidth} \centering \includegraphics[width = \textwidth]{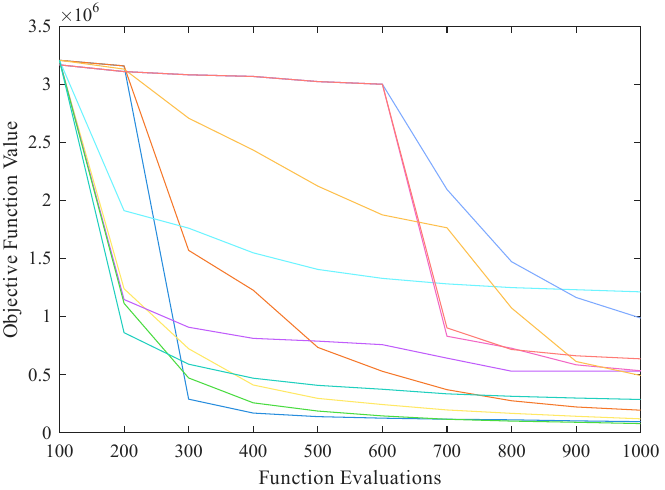} \\ F9 \end{minipage}
    \begin{minipage}[t]{0.195\textwidth} \centering \includegraphics[width = \textwidth]{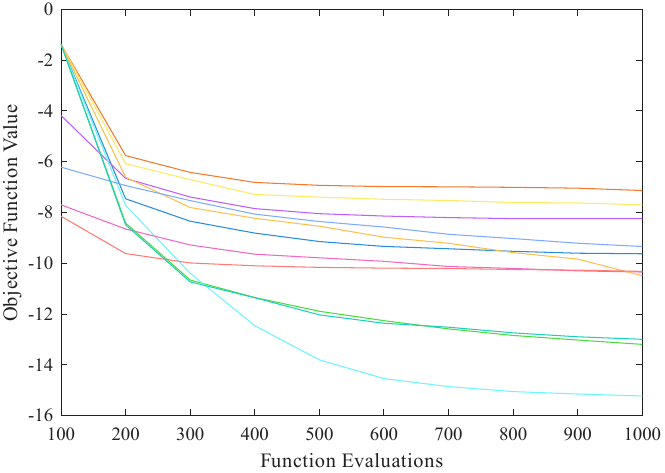} \\ F10 \end{minipage}
    \\\vspace{4mm}
    \begin{minipage}[t]{0.195\textwidth} \centering \includegraphics[width = \textwidth]{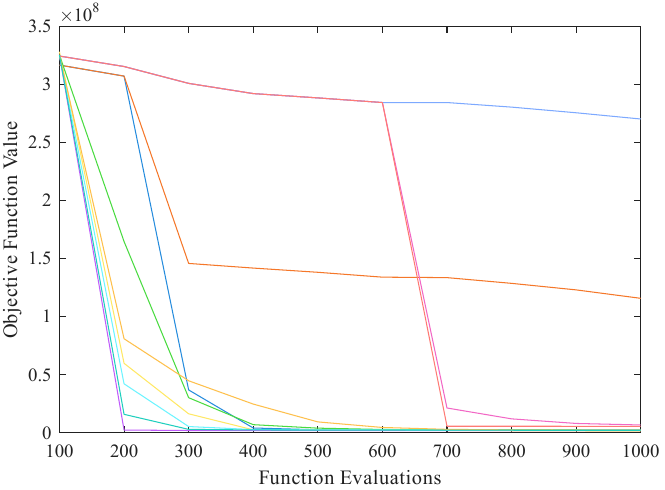} \\ F11-1 \end{minipage}
    \begin{minipage}[t]{0.195\textwidth} \centering \includegraphics[width = \textwidth]{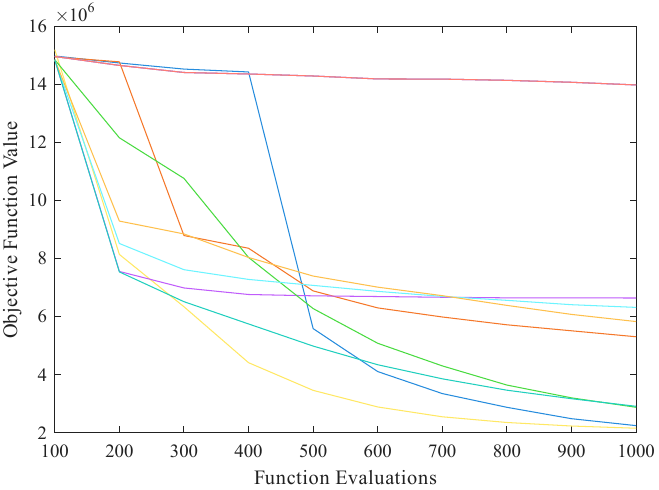} \\ F11-2 \end{minipage}
    \begin{minipage}[t]{0.195\textwidth} \centering \includegraphics[width = \textwidth]{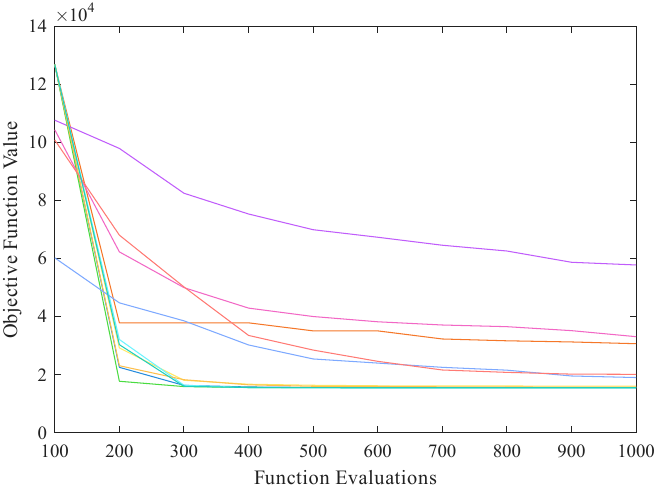} \\ F11-3 \end{minipage}
    \begin{minipage}[t]{0.195\textwidth} \centering \includegraphics[width = \textwidth]{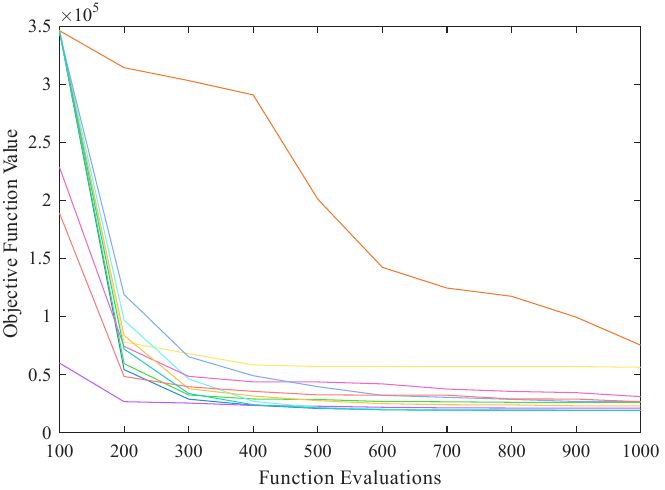} \\ F11-4 \end{minipage}
    \\\vspace{4mm}
    \begin{minipage}[t]{0.195\textwidth} \centering \includegraphics[width = \textwidth]{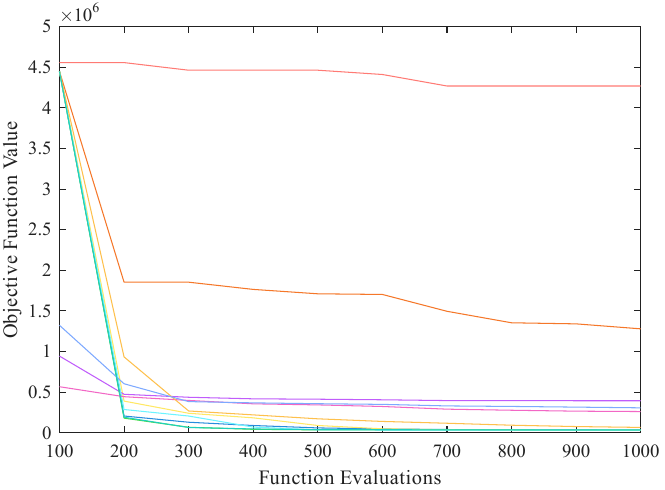} \\ F11-5 \end{minipage}
    \begin{minipage}[t]{0.195\textwidth} \centering \includegraphics[width = \textwidth]{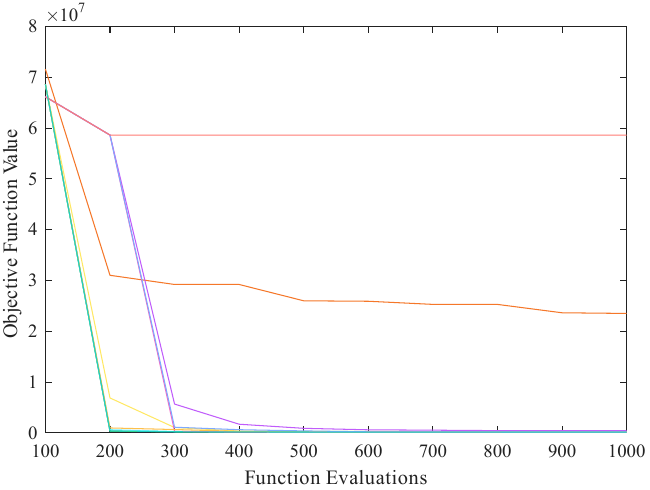} \\ F11-6 \end{minipage}
    \begin{minipage}[t]{0.195\textwidth} \centering \includegraphics[width = \textwidth]{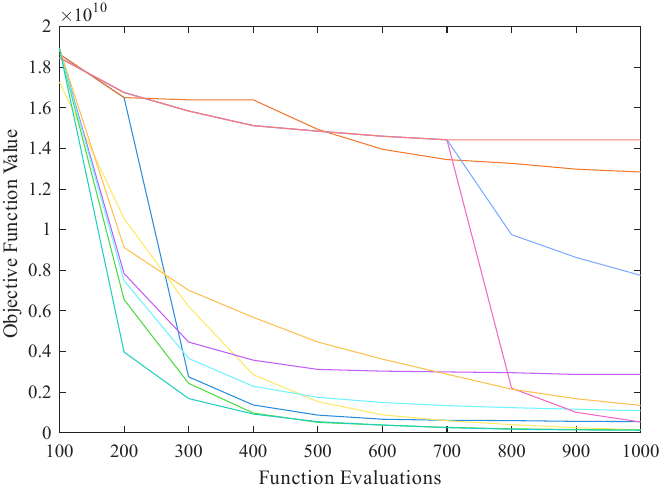} \\ F11-7 \end{minipage}
    \begin{minipage}[t]{0.195\textwidth} \centering \includegraphics[width = \textwidth]{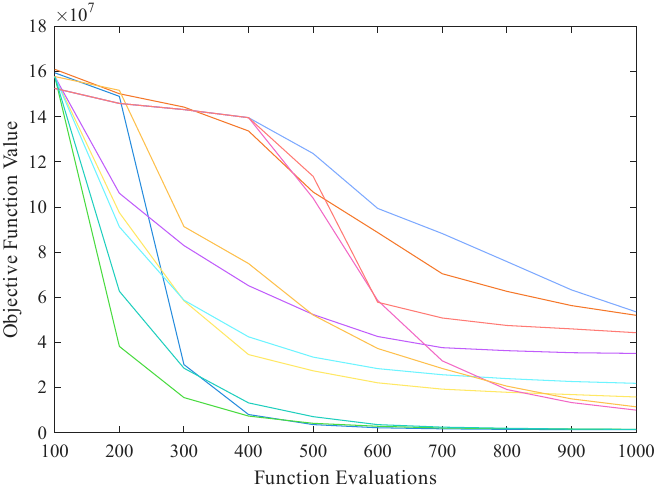} \\ F11-8 \end{minipage}
    \\\vspace{4mm}
    \begin{minipage}[t]{0.195\textwidth} \centering \includegraphics[width = \textwidth]{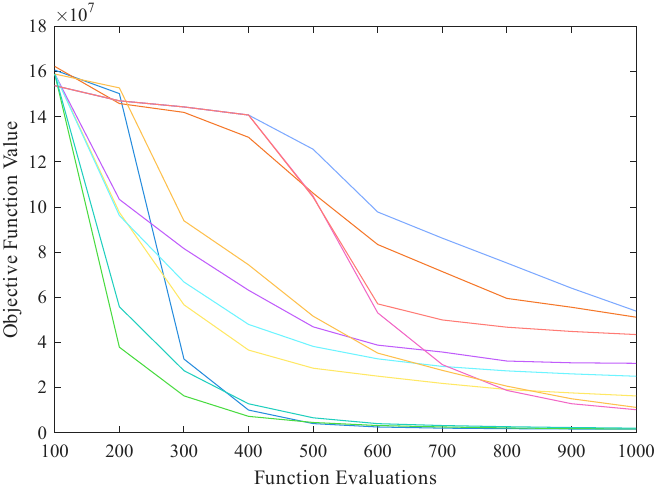} \\ F11-9 \end{minipage}
    \begin{minipage}[t]{0.195\textwidth} \centering \includegraphics[width = \textwidth]{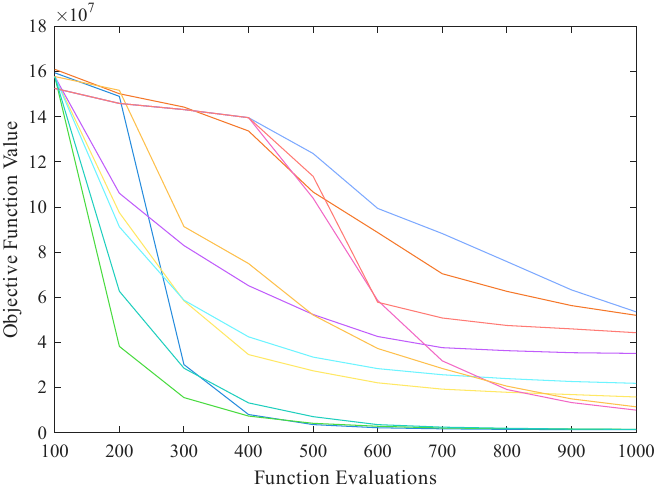} \\ F11-10 \end{minipage}
    \begin{minipage}[t]{0.195\textwidth} \centering \includegraphics[width = \textwidth]{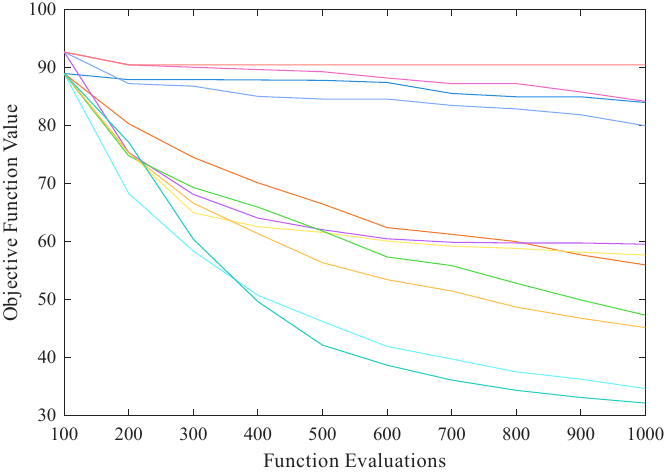} \\ F12 \end{minipage}
    \begin{minipage}[t]{0.195\textwidth} \centering \includegraphics[width = \textwidth]{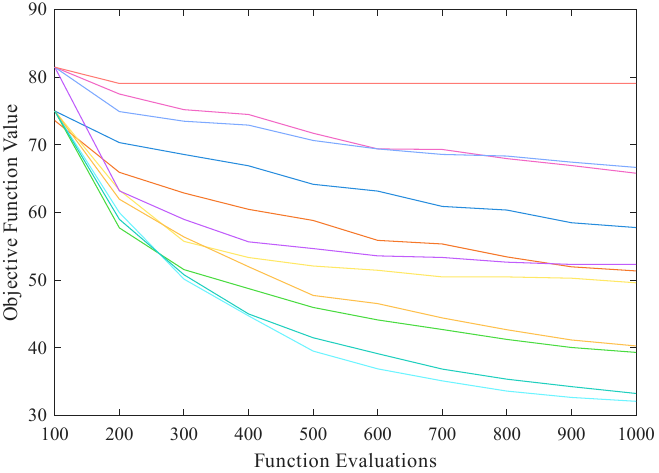} \\ F13 \end{minipage}
    \\\vspace{3mm}
    \caption{The convergence curves obtained in the experiments on the CEC2011 Real-world Problem Suite in Section~\ref{sec:dis-RW}.}
    \label{fig:convergence_curve_CEC2011RW}
\end{figure*}




% if have a single appendix:
%\appendix[Proof of the Zonklar Equations]
% or
%\appendix  % for no appendix heading
% do not use \section anymore after \appendix, only \section*
% is possibly needed

% use appendices with more than one appendix
% then use \section to start each appendix
% you must declare a \section before using any
% \subsection or using \label (\appendices by itself
% starts a section numbered zero.)
%


%\appendices
%\section{Proof of the First Zonklar Equation}
%Appendix one text goes here.

% you can choose not to have a title for an appendix
% if you want by leaving the argument blank
%\section{}
%Appendix two text goes here.


% use section* for acknowledgment
% \section*{Acknowledgment}

%The authors would like to thank...


% Can use something like this to put references on a page
% by themselves when using endfloat and the captionsoff option.
\ifCLASSOPTIONcaptionsoff
  \newpage
\fi



% trigger a \newpage just before the given reference
% number - used to balance the columns on the last page
% adjust value as needed - may need to be readjusted if
% the document is modified later
%\IEEEtriggeratref{8}
% The "triggered" command can be changed if desired:
%\IEEEtriggercmd{\enlargethispage{-5in}}

% references section

% can use a bibliography generated by BibTeX as a .bbl file
% BibTeX documentation can be easily obtained at:
% http://mirror.ctan.org/biblio/bibtex/contrib/doc/
% The IEEEtran BibTeX style support page is at:
% http://www.michaelshell.org/tex/ieeetran/bibtex/
%\bibliographystyle{IEEEtran}
% argument is your BibTeX string definitions and bibliography database(s)
%\bibliography{IEEEabrv,../bib/paper}
%
% <OR> manually copy in the resultant .bbl file
% set second argument of \begin to the number of references
% (used to reserve space for the reference number labels box)

% \bibliographystyle{IEEEtran}
% \input{main.bbl}
% \bibliography{myref}

%\begin{thebibliography}{1}
%\end{thebibliography}

% biography section
% 
% If you have an EPS/PDF photo (graphicx package needed) extra braces are
% needed around the contents of the optional argument to biography to prevent
% the LaTeX parser from getting confused when it sees the complicated
% \includegraphics command within an optional argument. (You could create
% your own custom macro containing the \includegraphics command to make things
% simpler here.)
%\begin{IEEEbiography}[{\includegraphics[width=1in,height=1.25in,clip,keepaspectratio]{mshell}}]{Michael Shell}
% or if you just want to reserve a space for a photo:


% You can push biographies down or up by placing
% a \vfill before or after them. The appropriate
% use of \vfill depends on what kind of text is
% on the last page and whether or not the columns
% are being equalized.

%\vfill

% Can be used to pull up biographies so that the bottom of the last one
% is flush with the other column.
%\enlargethispage{-5in}



% that's all folks
\end{document}
